# Supplementary material for: The Lothbrok approach for SPARQL Query Optimization over Decentralized Knowledge Graphs
Source: arXiv:2208.14692 source file (2022-08-31)
Supplement: Supplementary file 1 [file appendixb.tex]

In this appendix, we provide additional measures for the WatDiv shapes experiments.
Figure~\ref{fig:appb:nrf_nrn_bo} shows the number of relevant fragments (NRF) (Figures~\ref{subfig:appb:nrf_bo_10M}-\ref{subfig:appb:nrf_bo_1000M}) and nodes (NRN) (Figures~\ref{subfig:appb:nrn_bo_10M}-\ref{subfig:appb:nrn_bo_1000M}) \emph{before} optimization, and the number of nodes involved with processing each query (Figures~\ref{subfig:appb:niq_10M}-\ref{subfig:appb:niq_1000M}) including the nodes the nodes that subqueries were delegated to.
Furthermore, Figure~\ref{fig:appb:npf_npn} shows the number of pruned fragments (Figures~\ref{subfig:appb:npf_10M}-\ref{subfig:appb:npf_1000M}) and nodes (Figures~\ref{subfig:appb:npn_10M}-\ref{subfig:appb:npn_1000M}) per query.

\begin{figure*}[tb!]
\centering
\includegraphics[width=.6\textwidth]{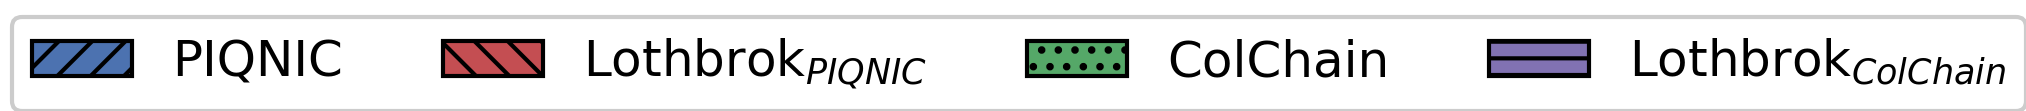}
\begin{subfigure}[b]{0.48\textwidth}
  \includegraphics[width=\textwidth]{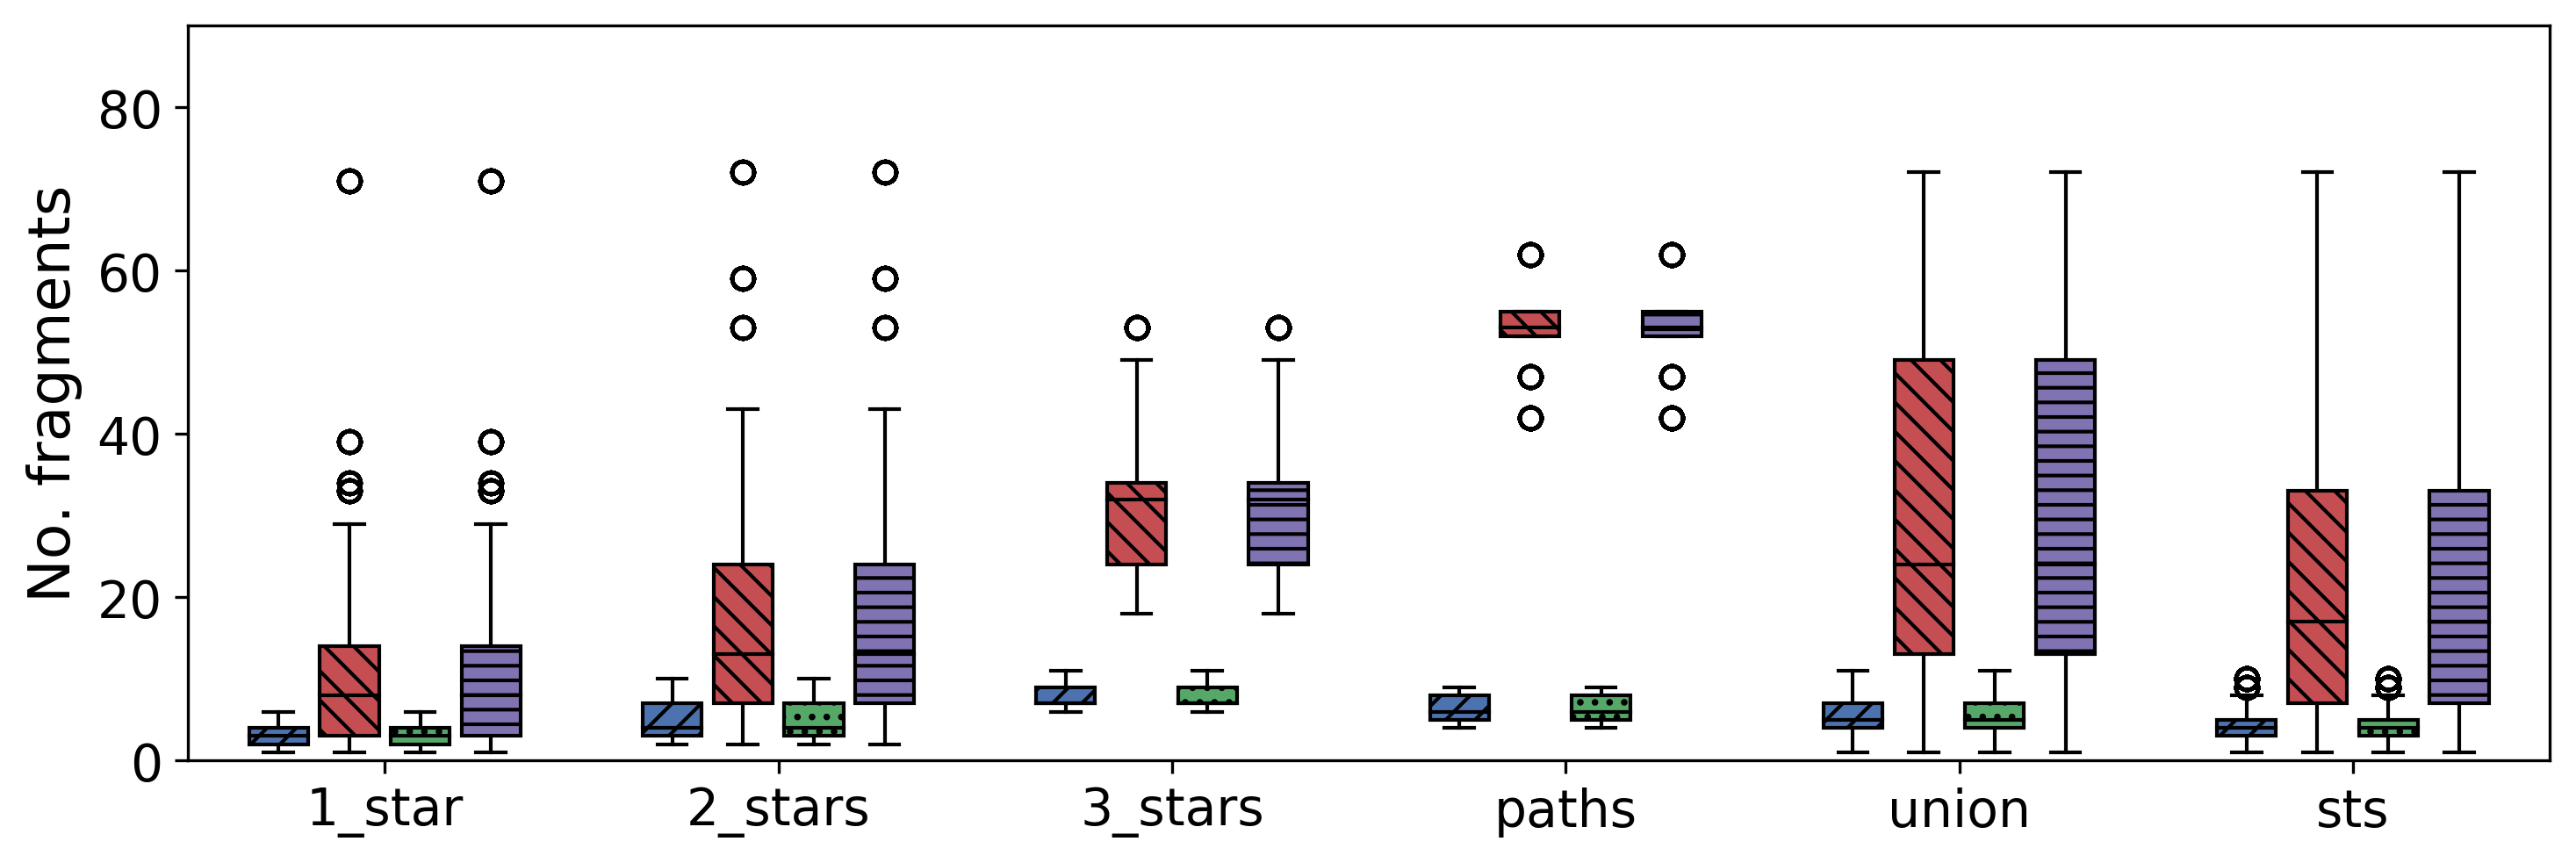}
  \caption{Number of relevant fragments (NRF) \emph{before} optimization over \texttt{watdiv10M}}\label{subfig:appb:nrf_bo_10M}
\end{subfigure}
\begin{subfigure}[b]{0.48\textwidth}
  \includegraphics[width=\textwidth]{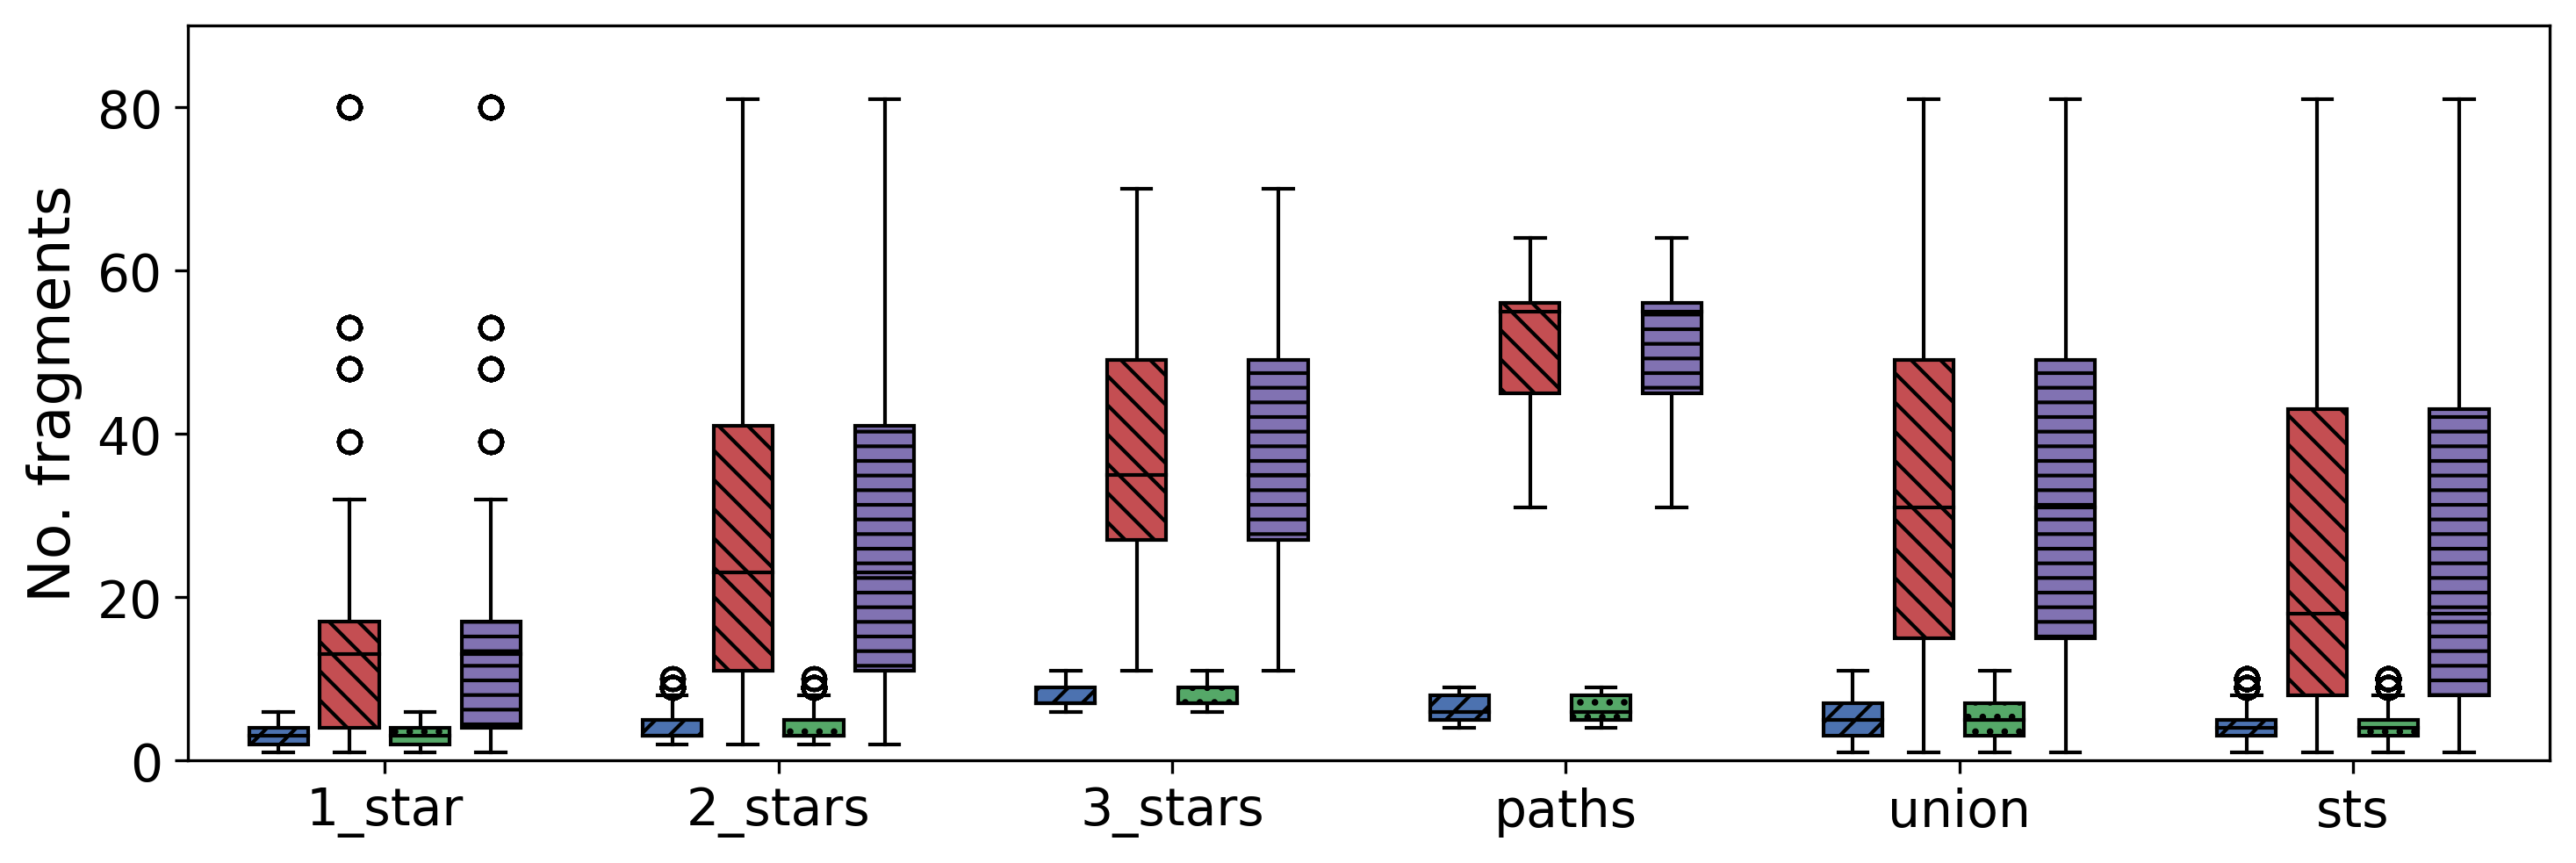}
  \caption{Number of relevant fragments (NRF) \emph{before} optimization over \texttt{watdiv100M}}\label{subfig:appb:nrf_bo_100M}
\end{subfigure}
\begin{subfigure}[b]{0.48\textwidth}
  \includegraphics[width=\textwidth]{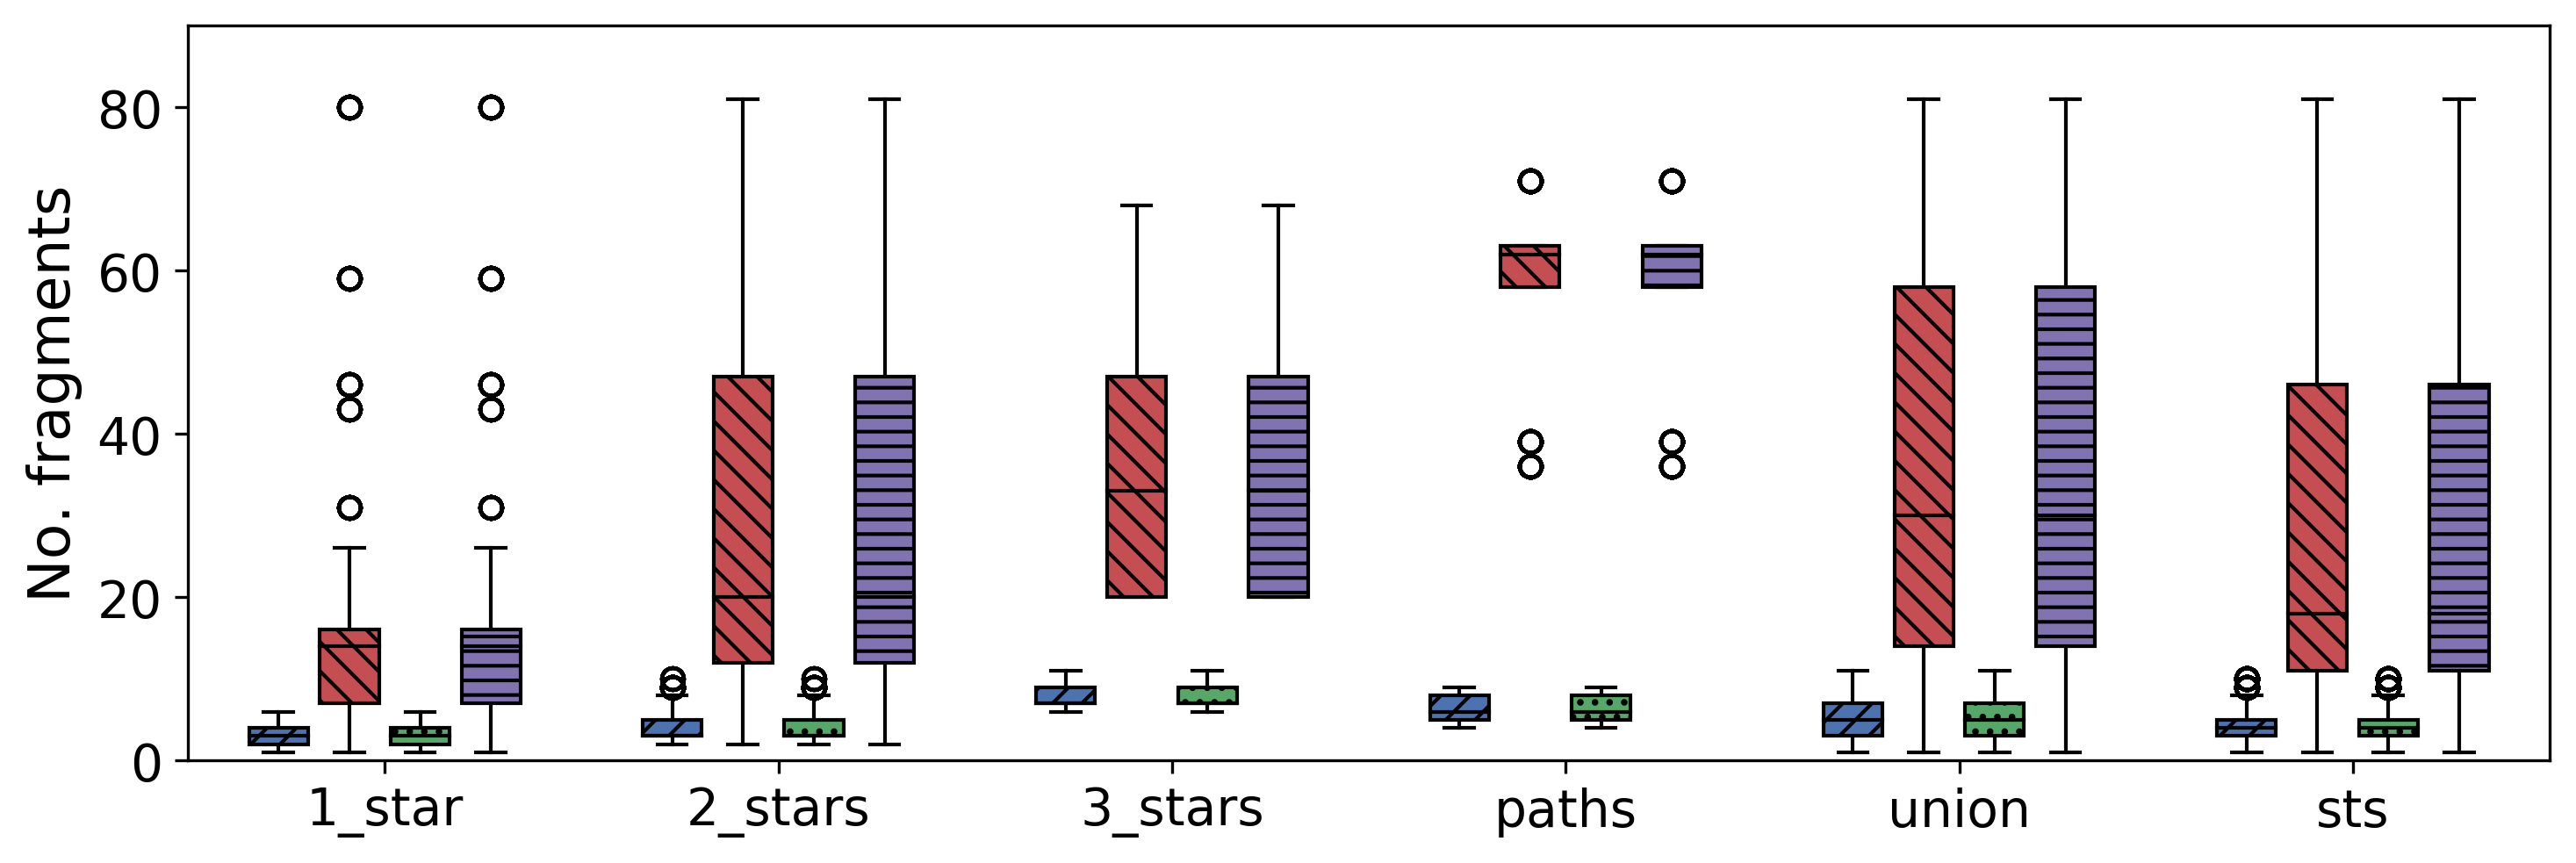}
  \caption{Number of relevant fragments (NRF) \emph{before} optimization over \texttt{watdiv1000M}}\label{subfig:appb:nrf_bo_1000M}
\end{subfigure}
\begin{subfigure}[b]{0.48\textwidth}
  \includegraphics[width=\textwidth]{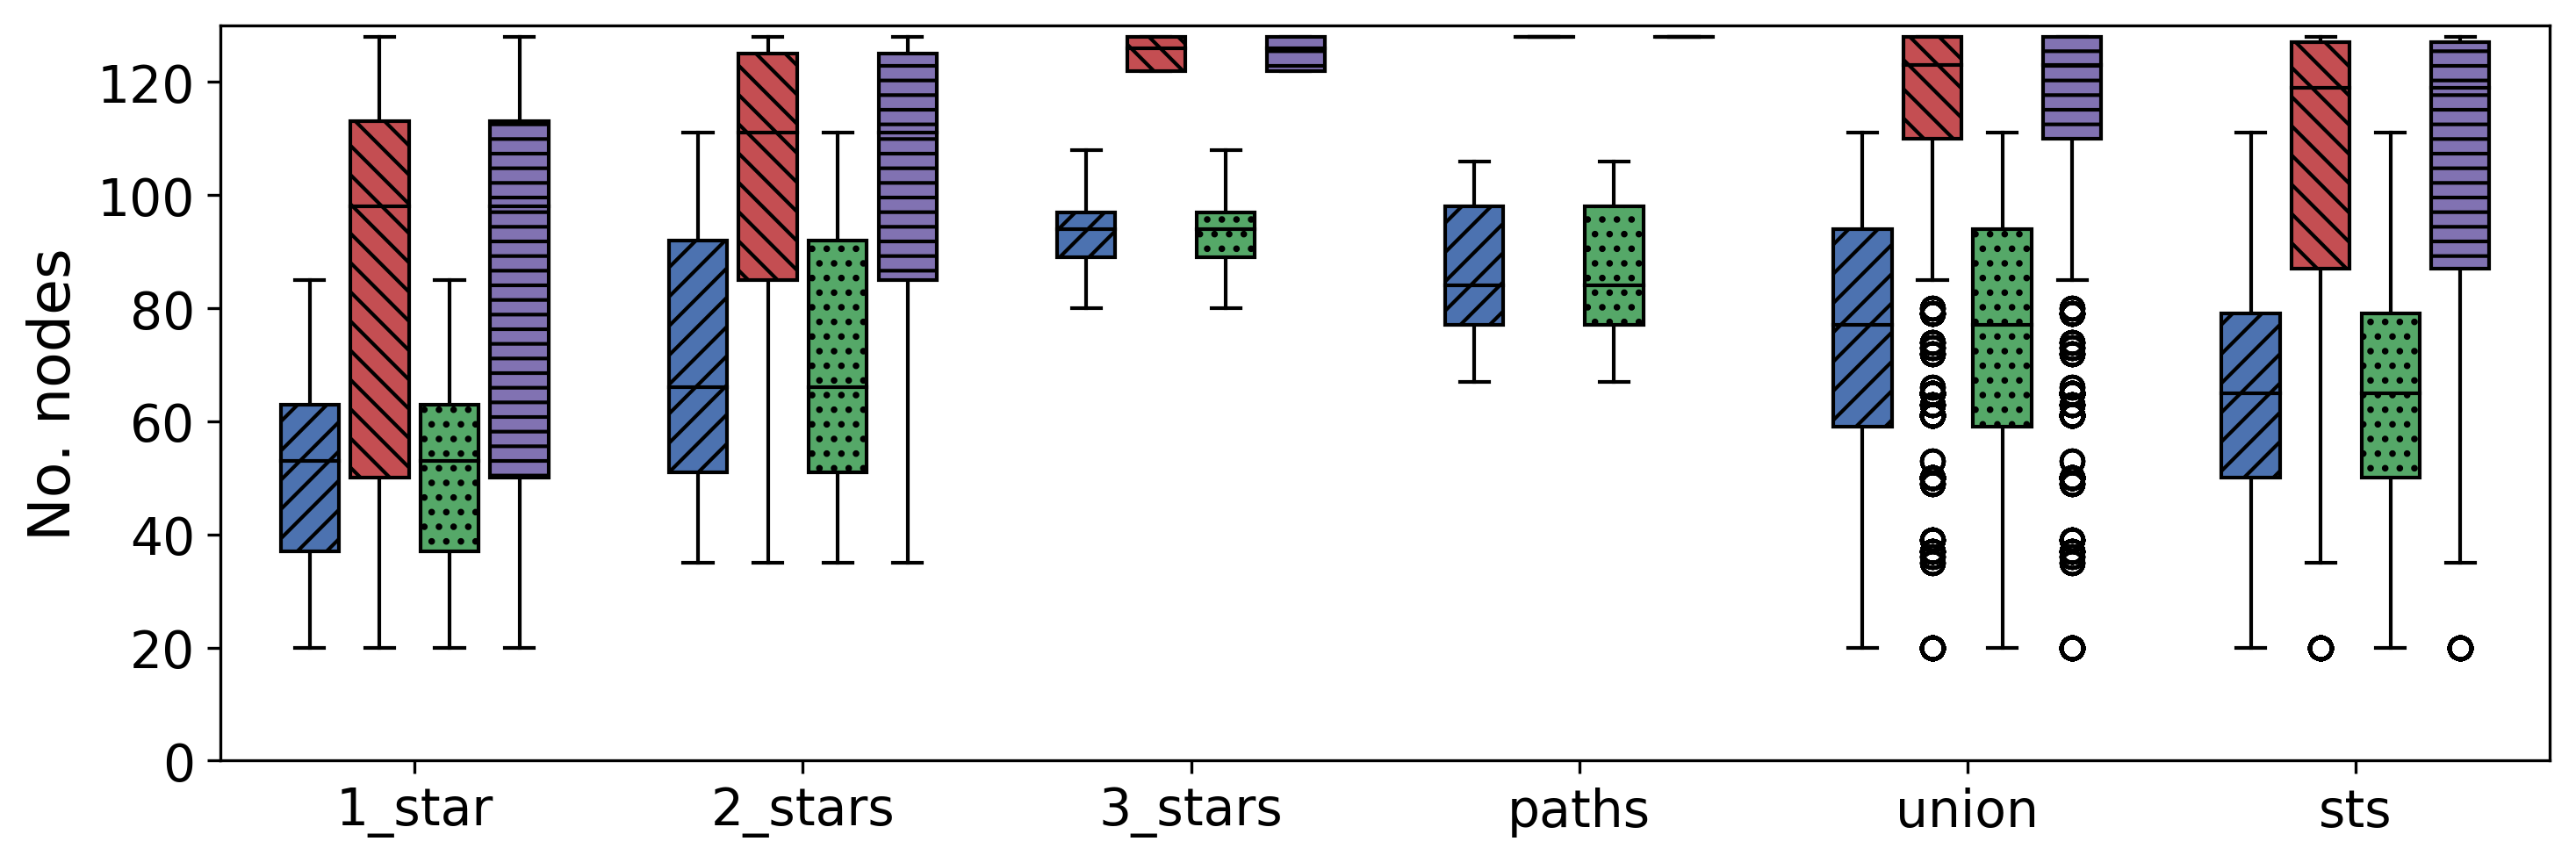}
  \caption{Number of relevant nodes (NRN) \emph{before} optimization over \texttt{watdiv10M}}\label{subfig:appb:nrn_bo_10M}
\end{subfigure}
\begin{subfigure}[b]{0.48\textwidth}
  \includegraphics[width=\textwidth]{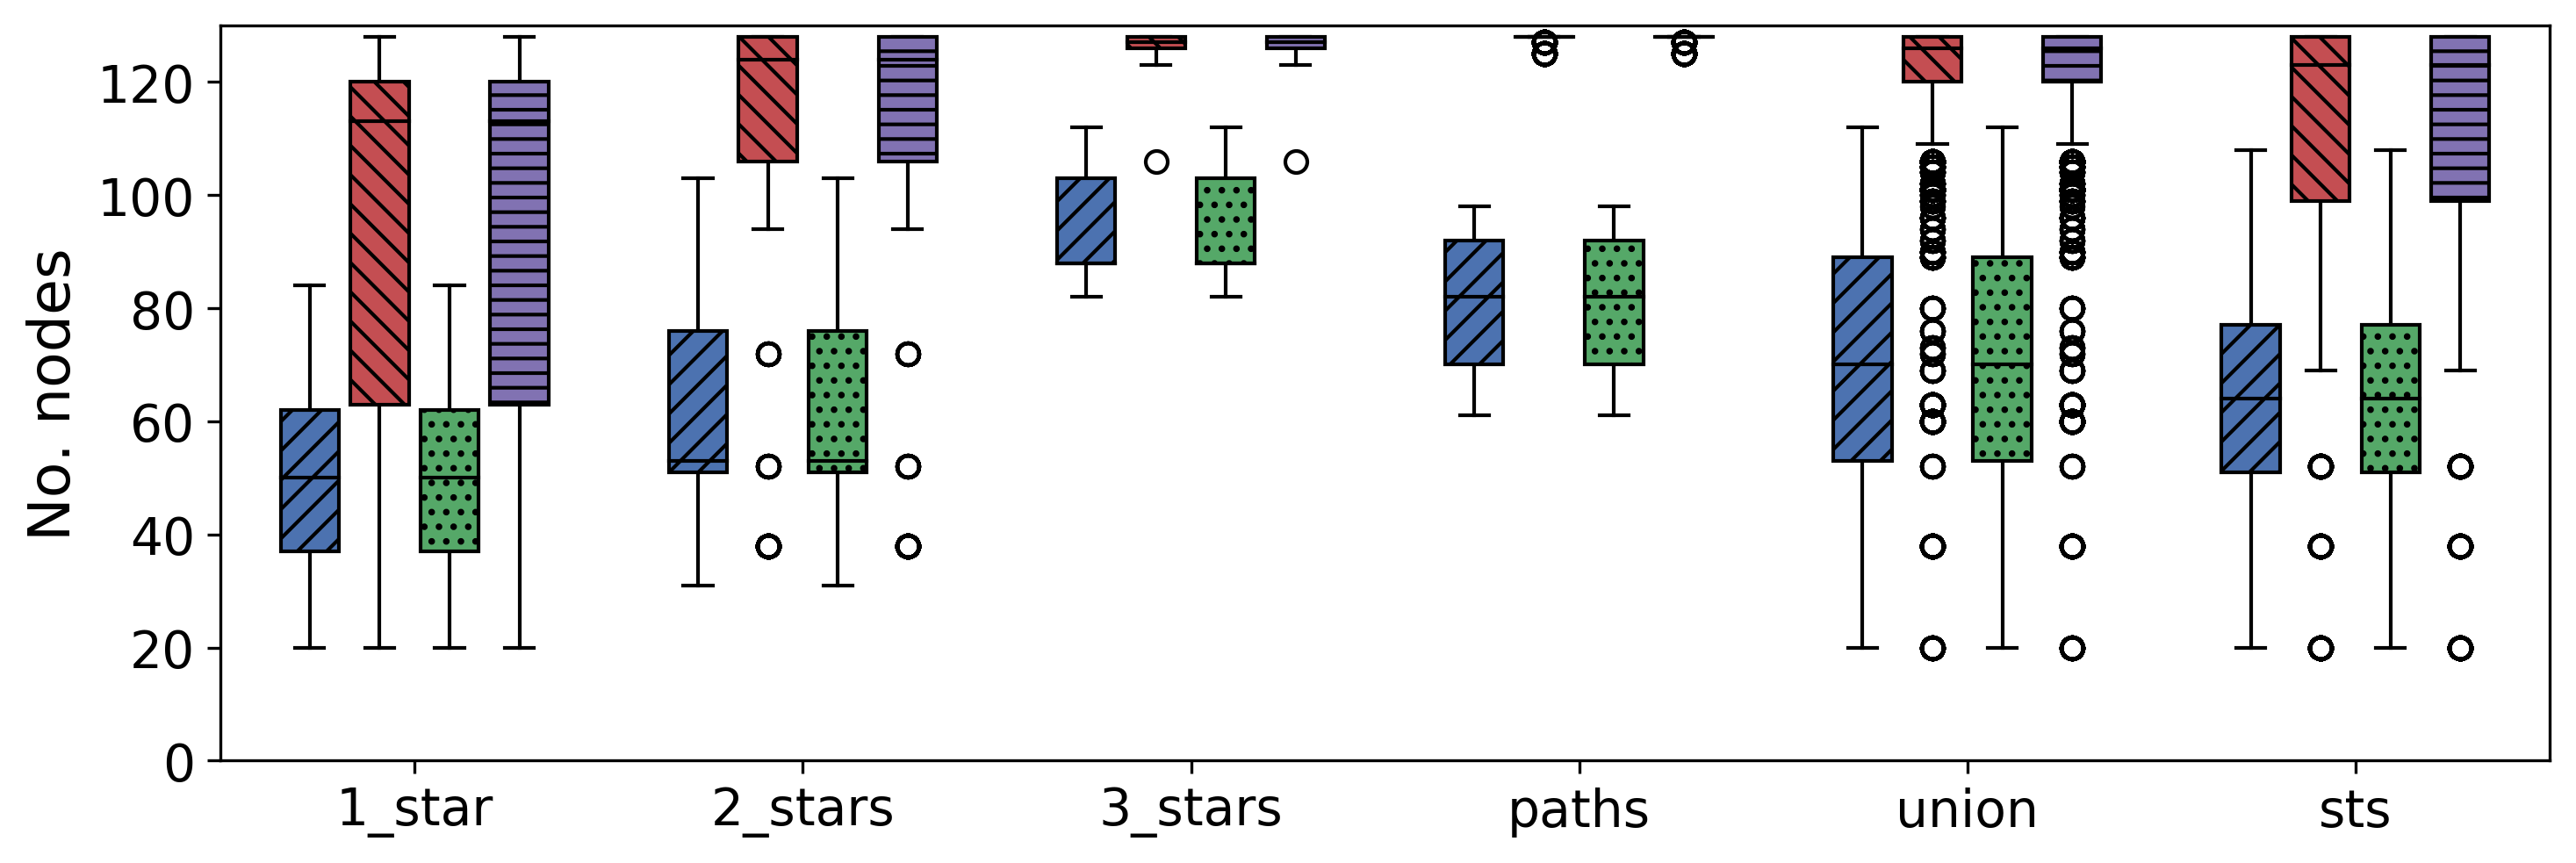}
  \caption{Number of relevant nodes (NRN) \emph{before} optimization over \texttt{watdiv100M}}\label{subfig:appb:nrn_bo_100M}
\end{subfigure}
\begin{subfigure}[b]{0.48\textwidth}
  \includegraphics[width=\textwidth]{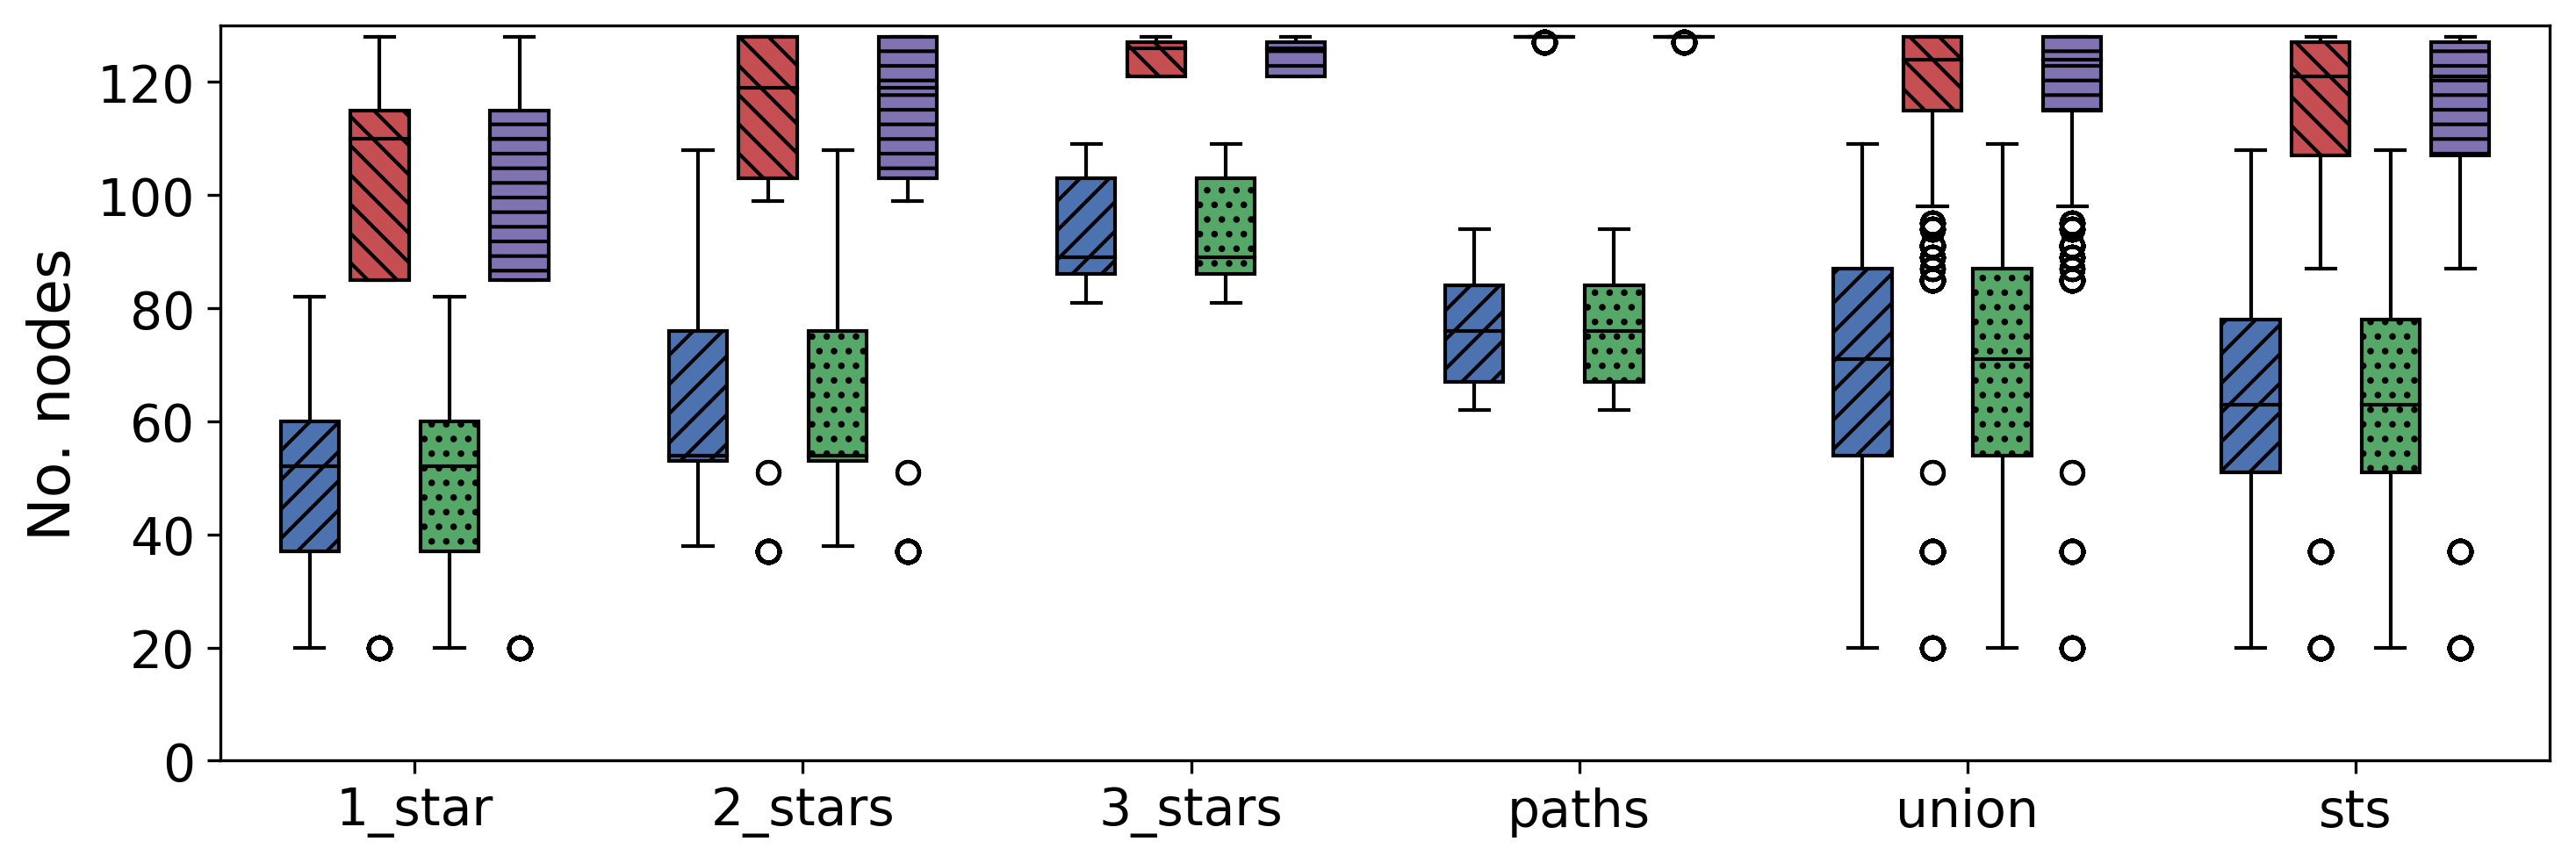}
  \caption{Number of relevant nodes (NRN) \emph{before} optimization over \texttt{watdiv1000M}}\label{subfig:appb:nrn_bo_1000M}
\end{subfigure}
\begin{subfigure}[b]{0.48\textwidth}
  \includegraphics[width=\textwidth]{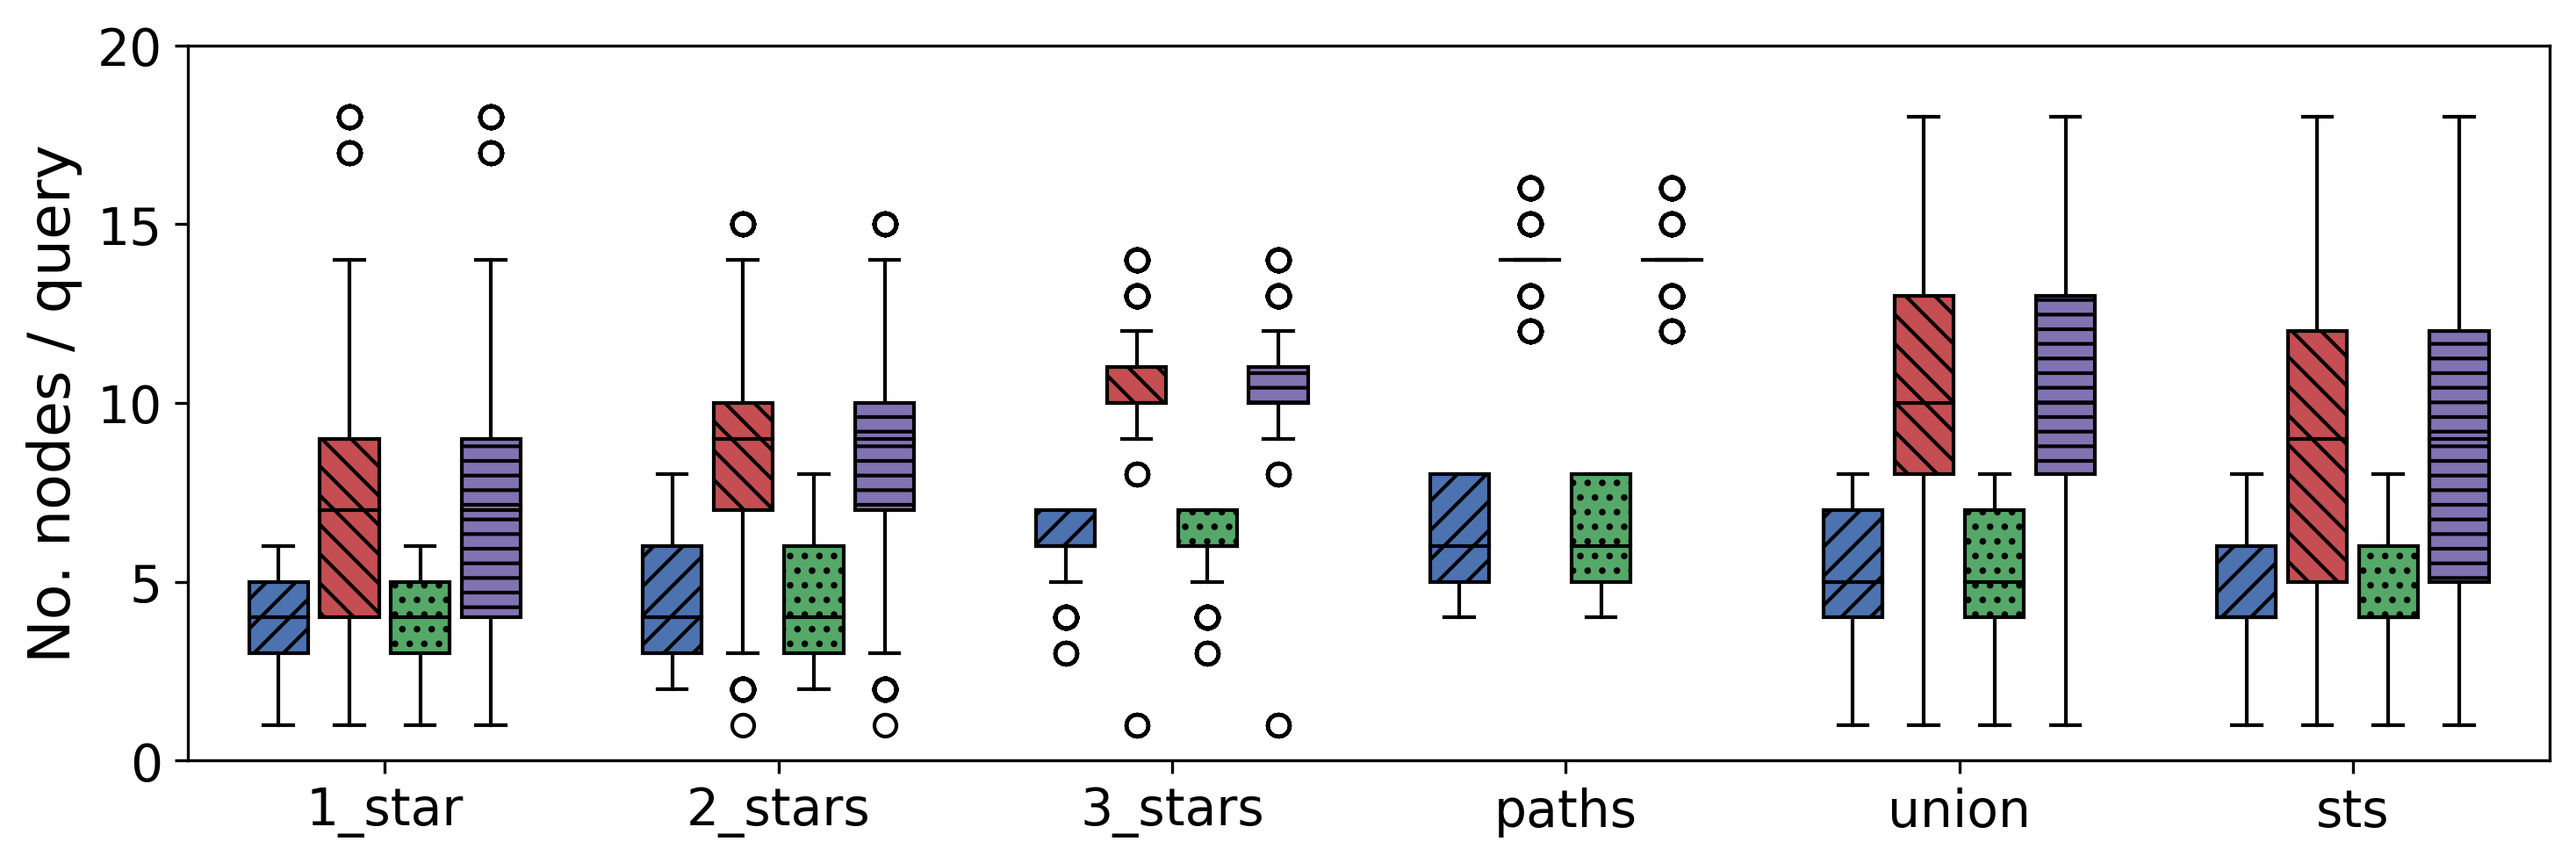}
  \caption{Number of involved nodes over \texttt{watdiv10M}}\label{subfig:appb:niq_10M}
\end{subfigure}
\begin{subfigure}[b]{0.48\textwidth}
  \includegraphics[width=\textwidth]{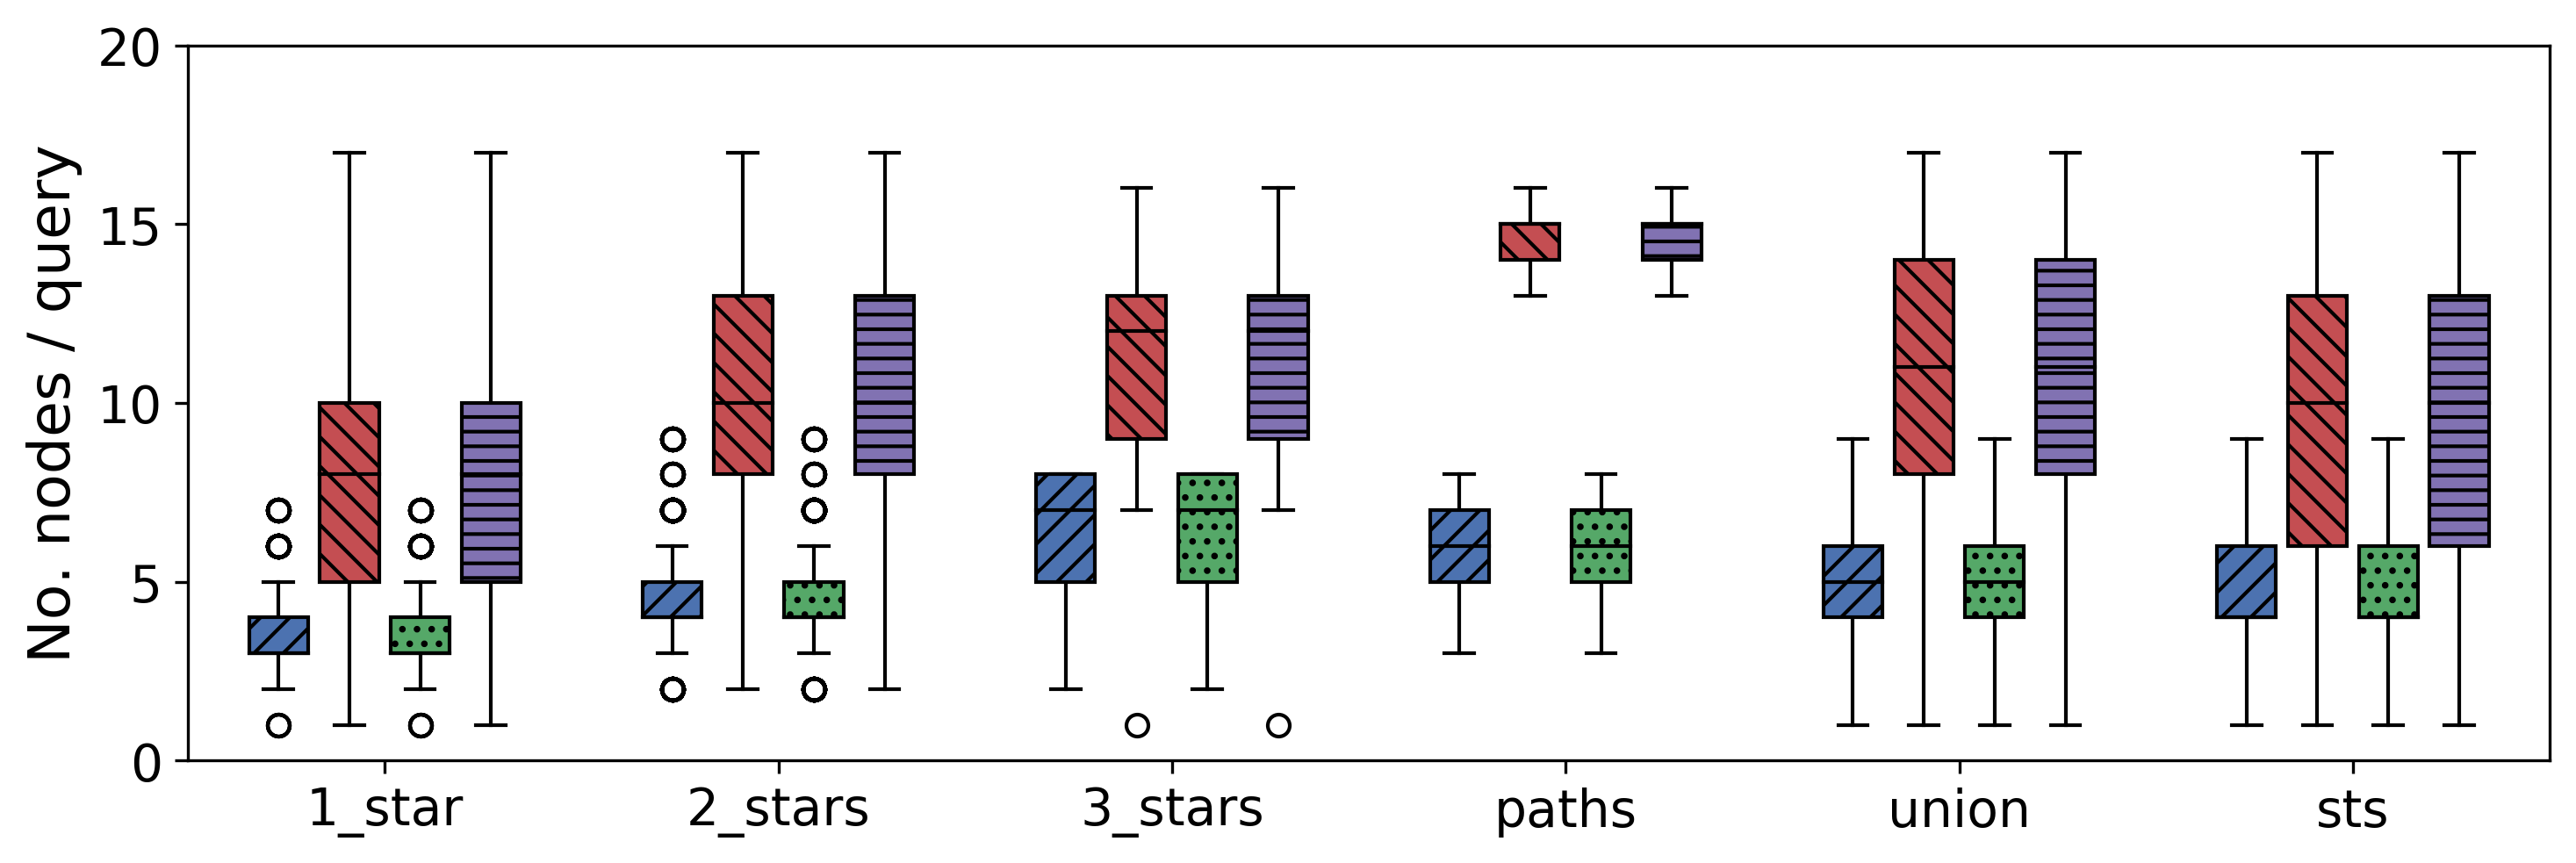}
  \caption{Number of involved nodes over \texttt{watdiv100M}}\label{subfig:appb:niq_100M}
\end{subfigure}
\begin{subfigure}[b]{0.48\textwidth}
  \includegraphics[width=\textwidth]{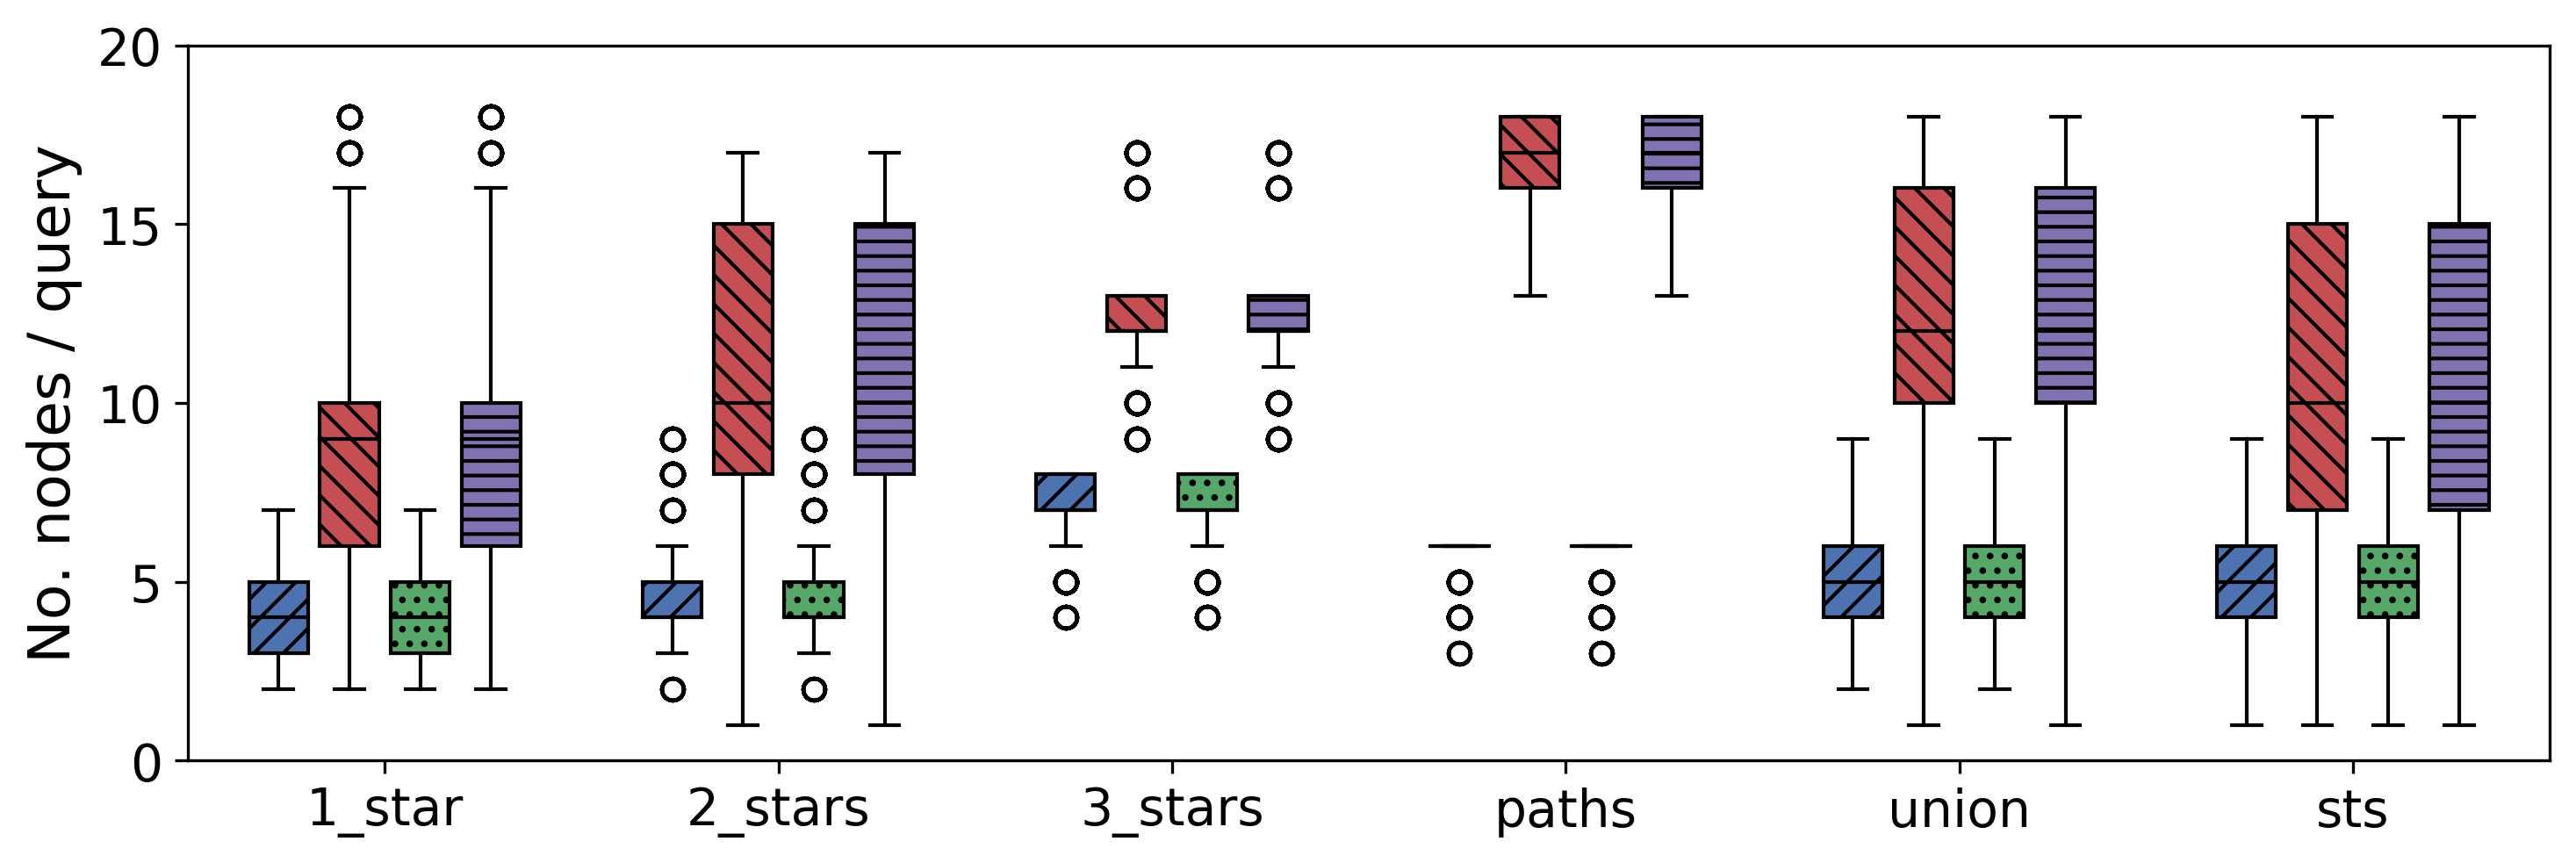}
  \caption{Number of involved nodes over \texttt{watdiv1000M}}\label{subfig:appb:niq_1000M}
\end{subfigure}
\caption{Number of relevant fragments (NRF) and nodes (NRN) \emph{before} optimization, and number of nodes involved with processing each query for the WatDiv datasets and star queries.}
\label{fig:appb:nrf_nrn_bo}
\end{figure*}

\begin{figure*}[tb!]
\centering
\begin{subfigure}[b]{0.48\textwidth}
  \includegraphics[width=\textwidth]{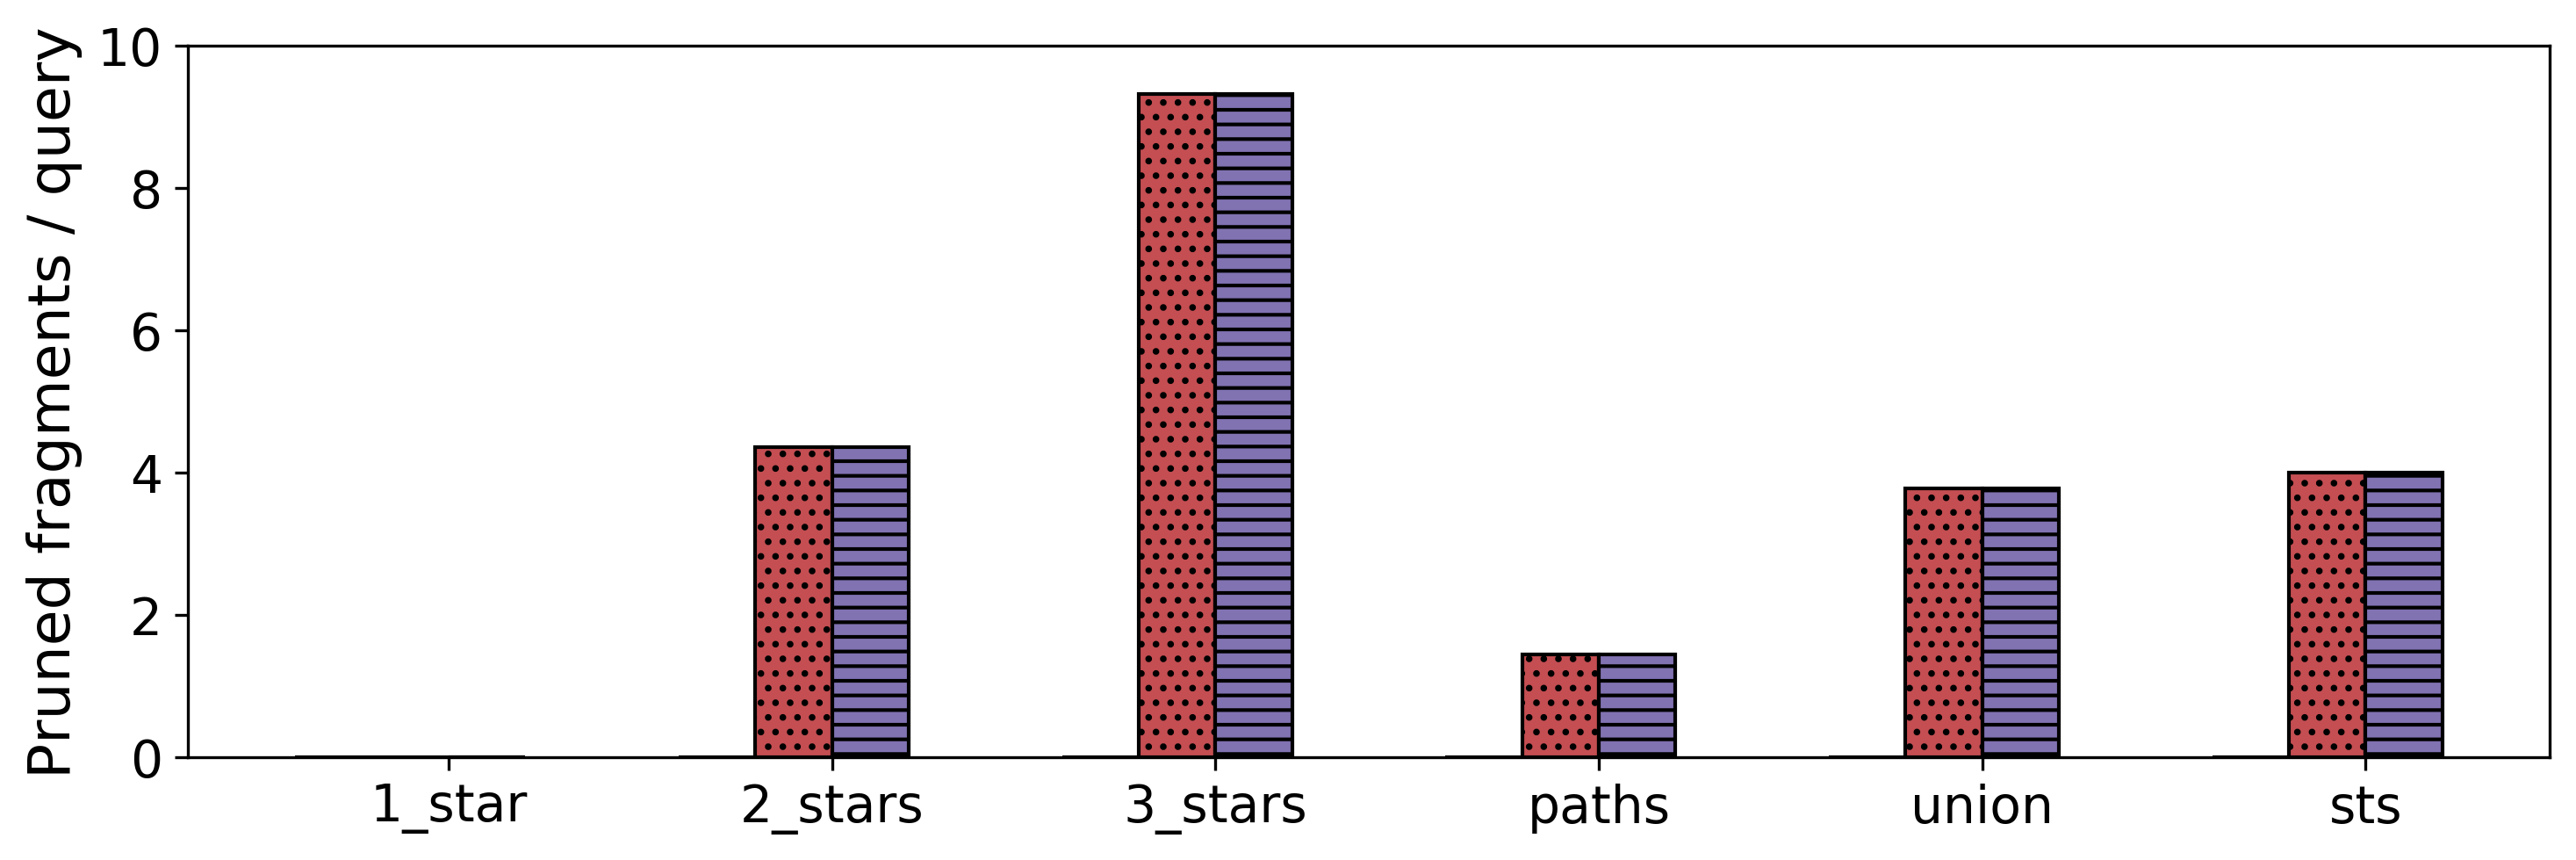}
  \caption{Number of pruned fragments per query over \texttt{watdiv10M}}\label{subfig:appb:npf_10M}
\end{subfigure}
\begin{subfigure}[b]{0.48\textwidth}
  \includegraphics[width=\textwidth]{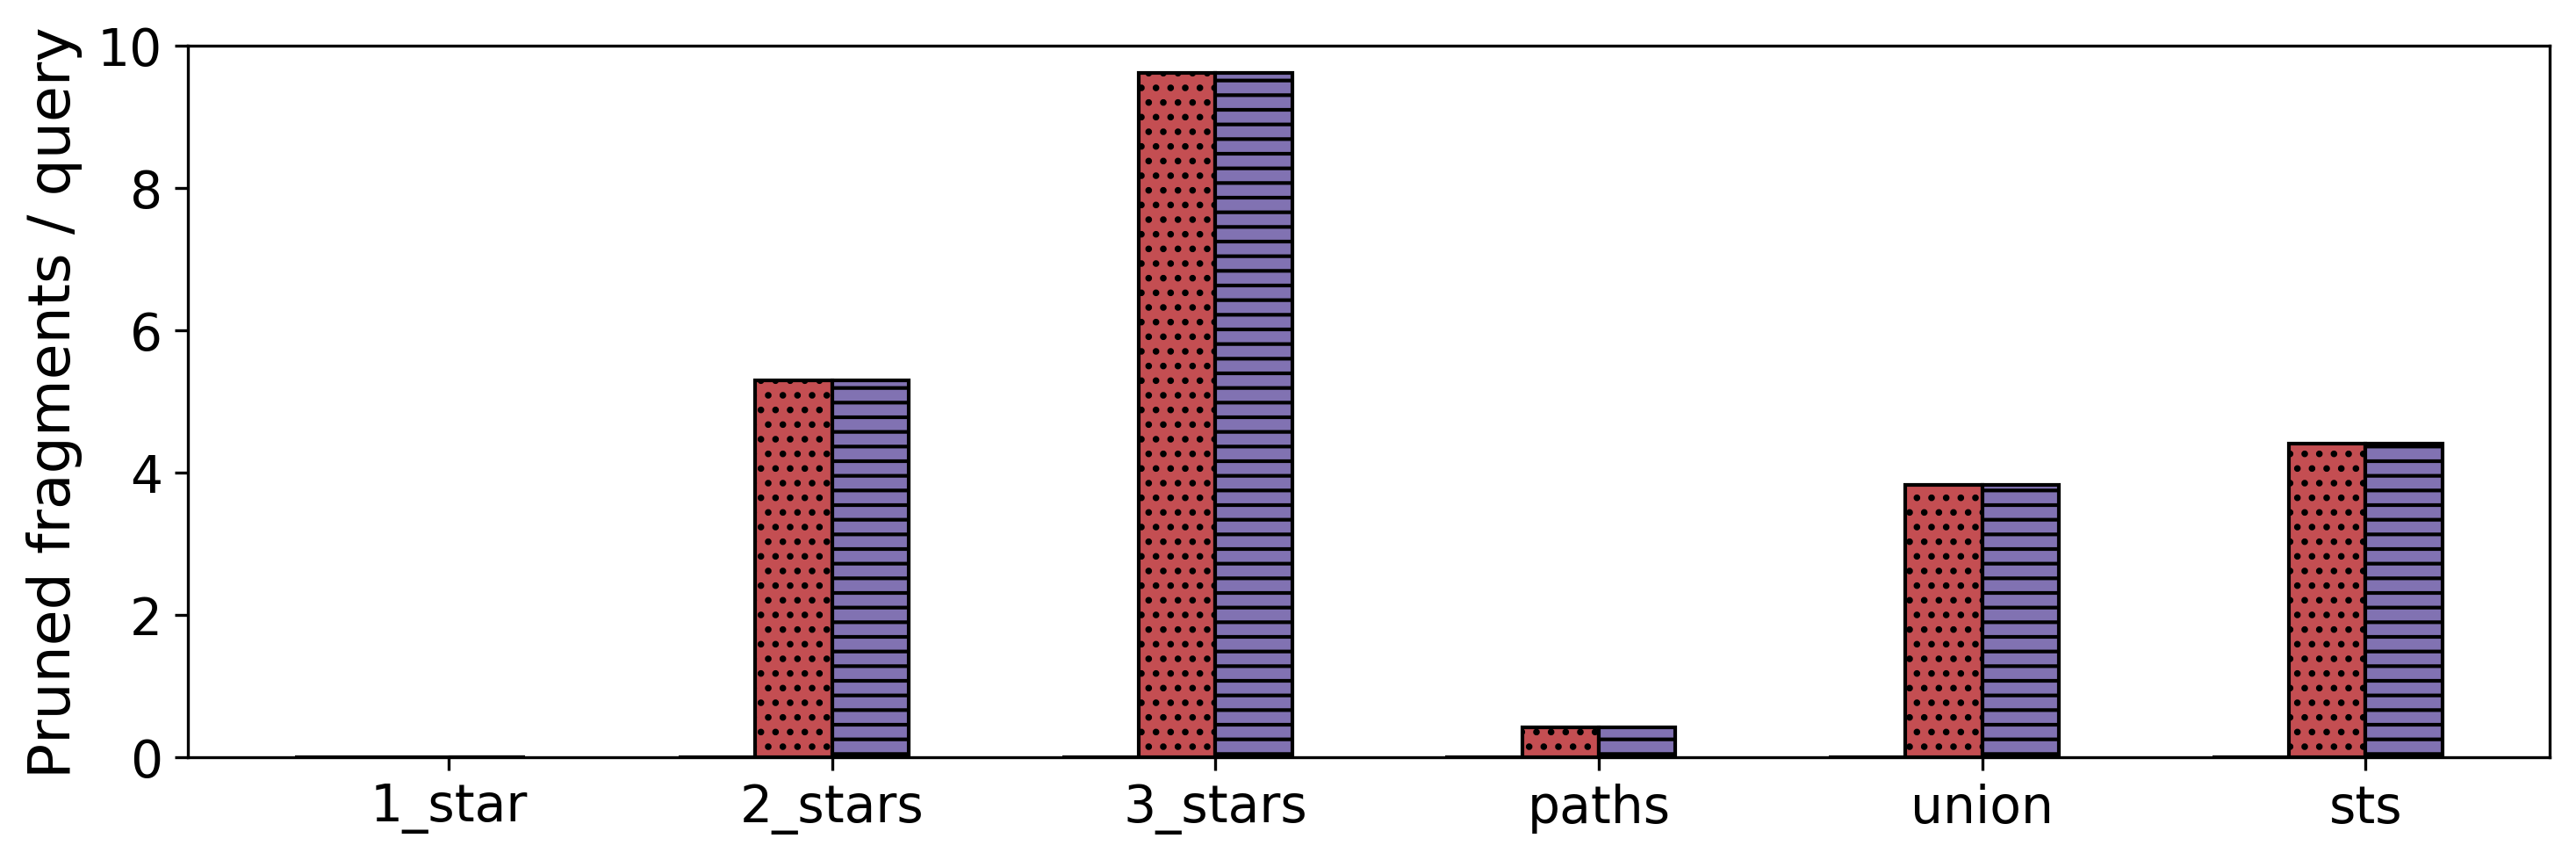}
  \caption{Number of pruned fragments per query over \texttt{watdiv100M}}\label{subfig:appb:npf_100M}
\end{subfigure}
\begin{subfigure}[b]{0.48\textwidth}
  \includegraphics[width=\textwidth]{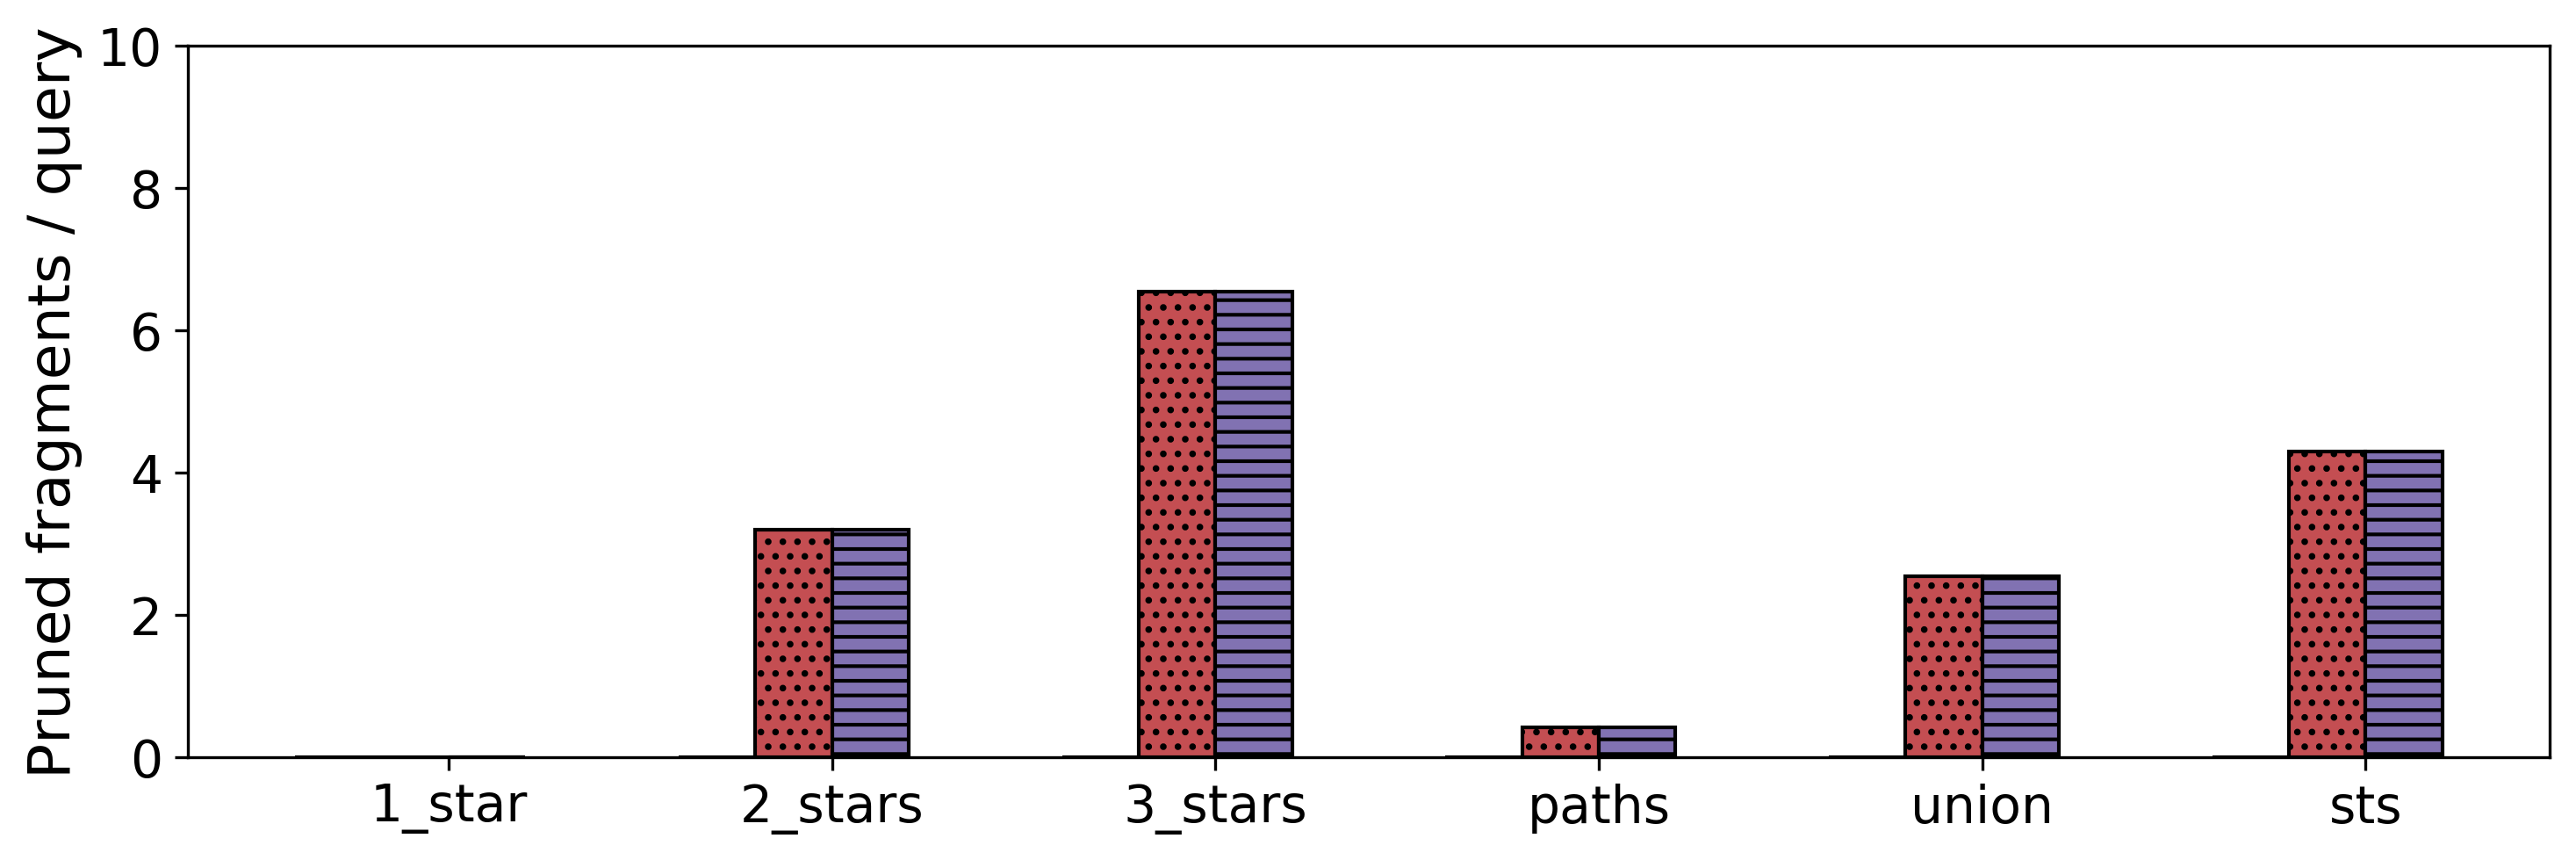}
  \caption{Number of pruned fragments per query over \texttt{watdiv1000M}}\label{subfig:appb:npf_1000M}
\end{subfigure}
\begin{subfigure}[b]{0.48\textwidth}
  \includegraphics[width=\textwidth]{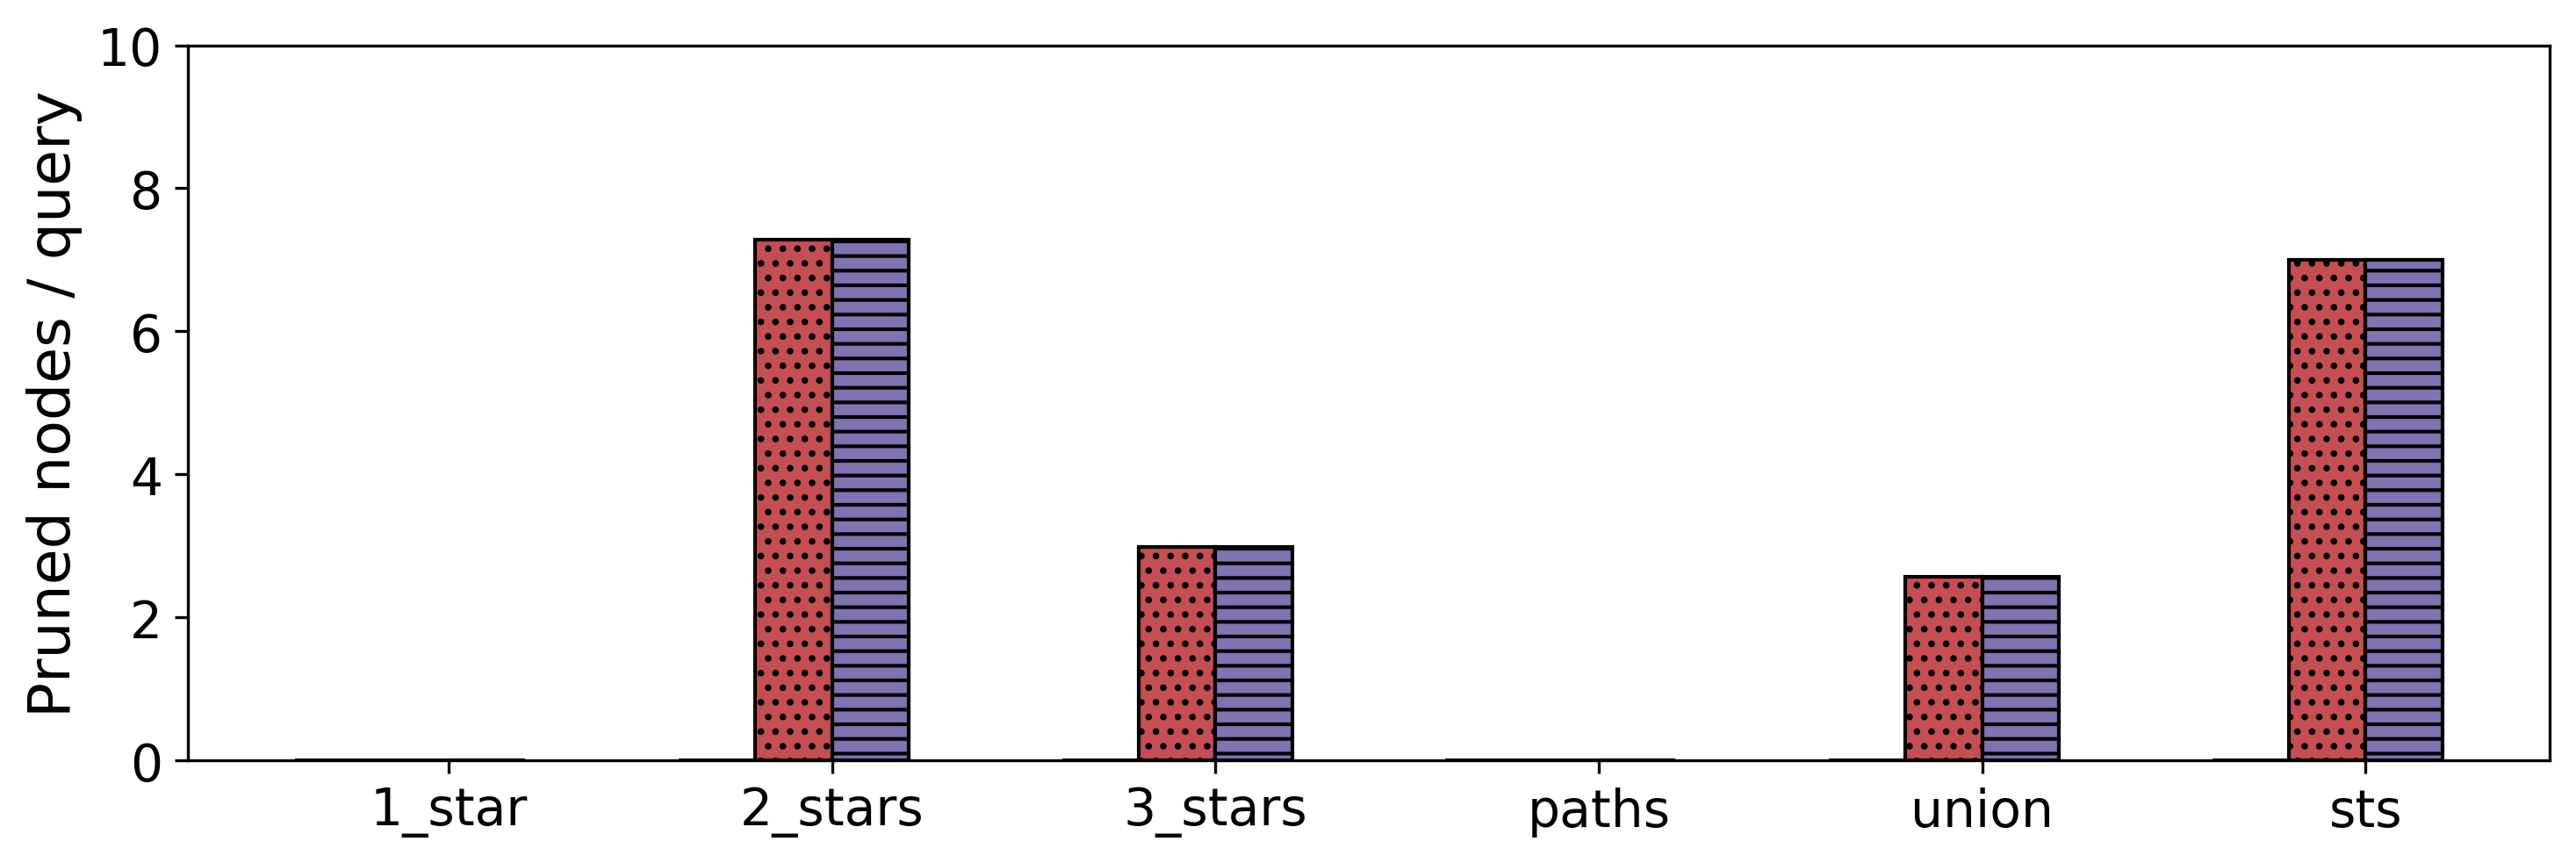}
  \caption{Number of pruned nodes per query over \texttt{watdiv10M}}\label{subfig:appb:npn_10M}
\end{subfigure}
\begin{subfigure}[b]{0.48\textwidth}
  \includegraphics[width=\textwidth]{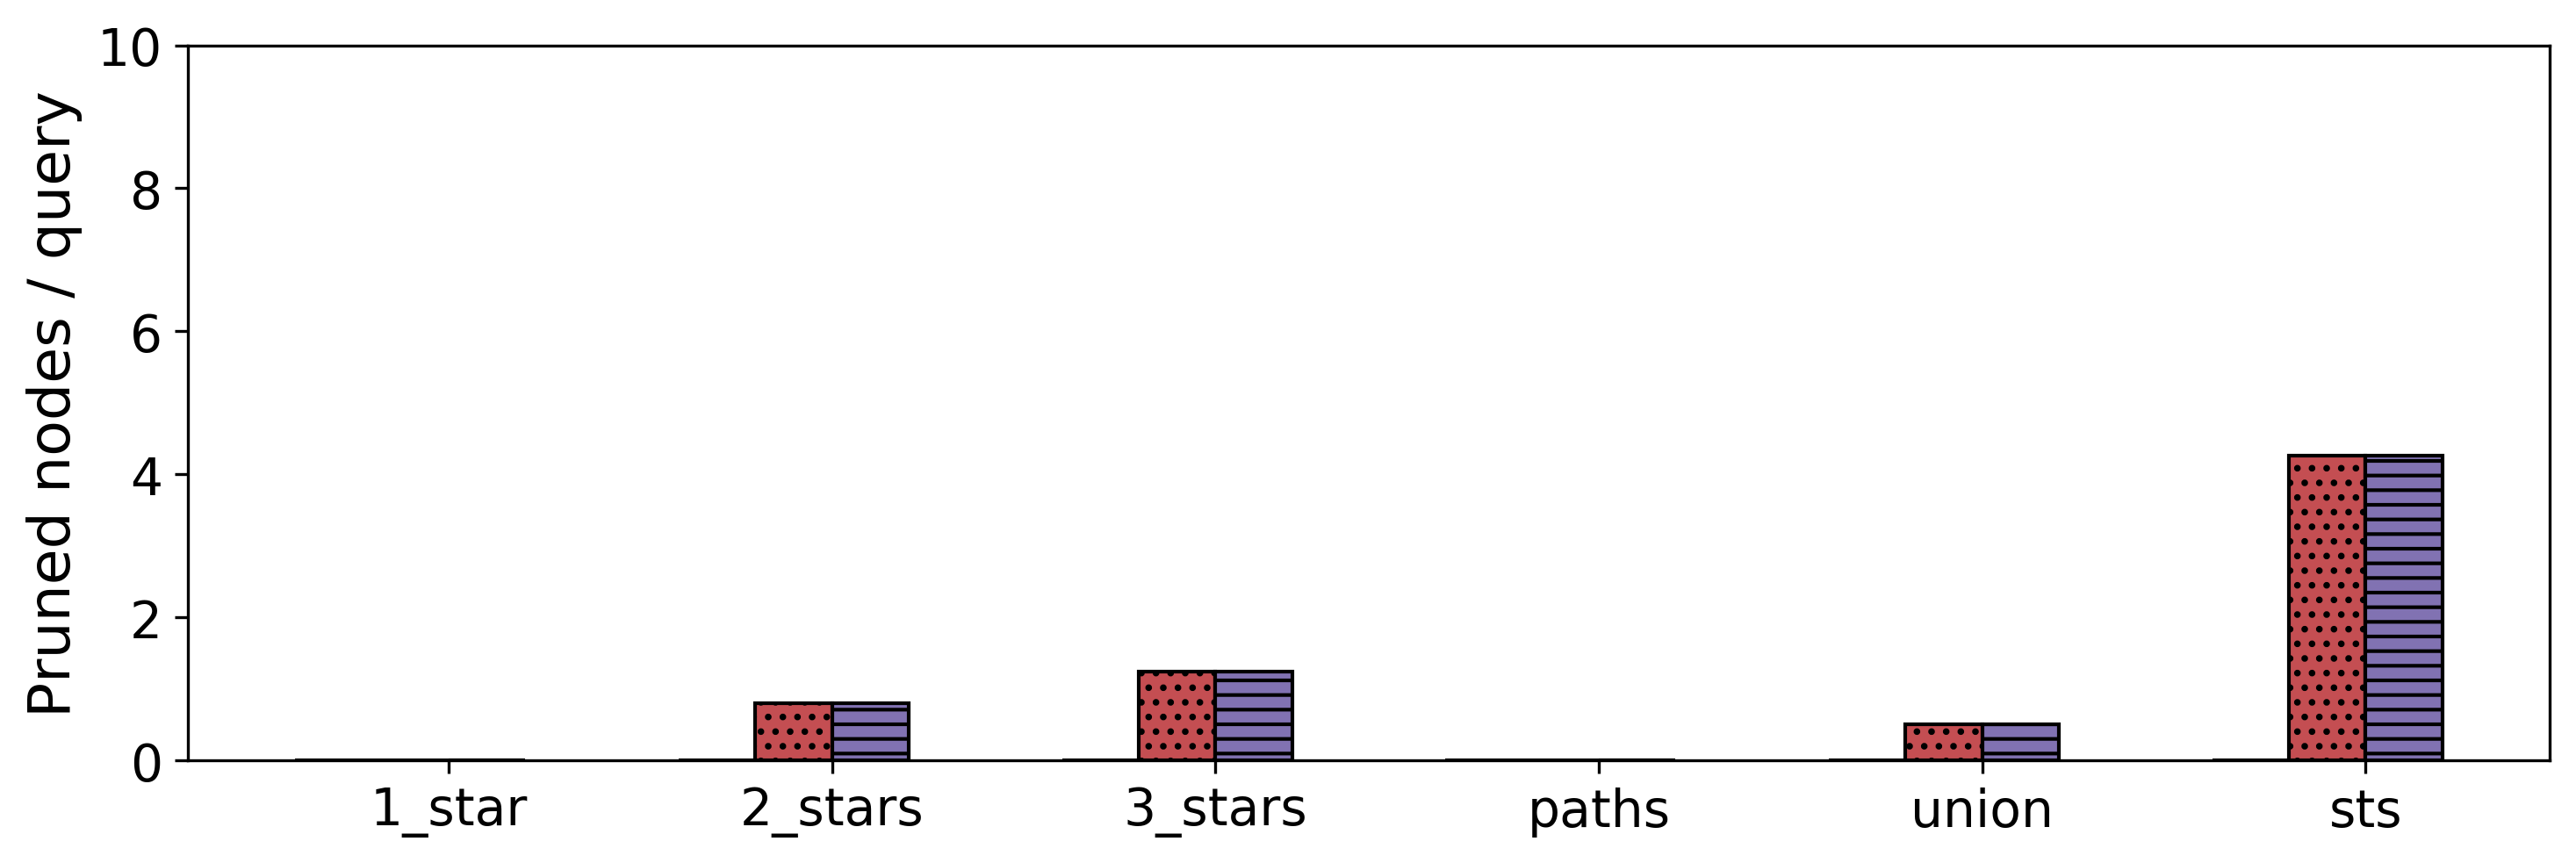}
  \caption{Number of pruned nodes per query over \texttt{watdiv100M}}\label{subfig:appb:npn_100M}
\end{subfigure}
\begin{subfigure}[b]{0.48\textwidth}
  \includegraphics[width=\textwidth]{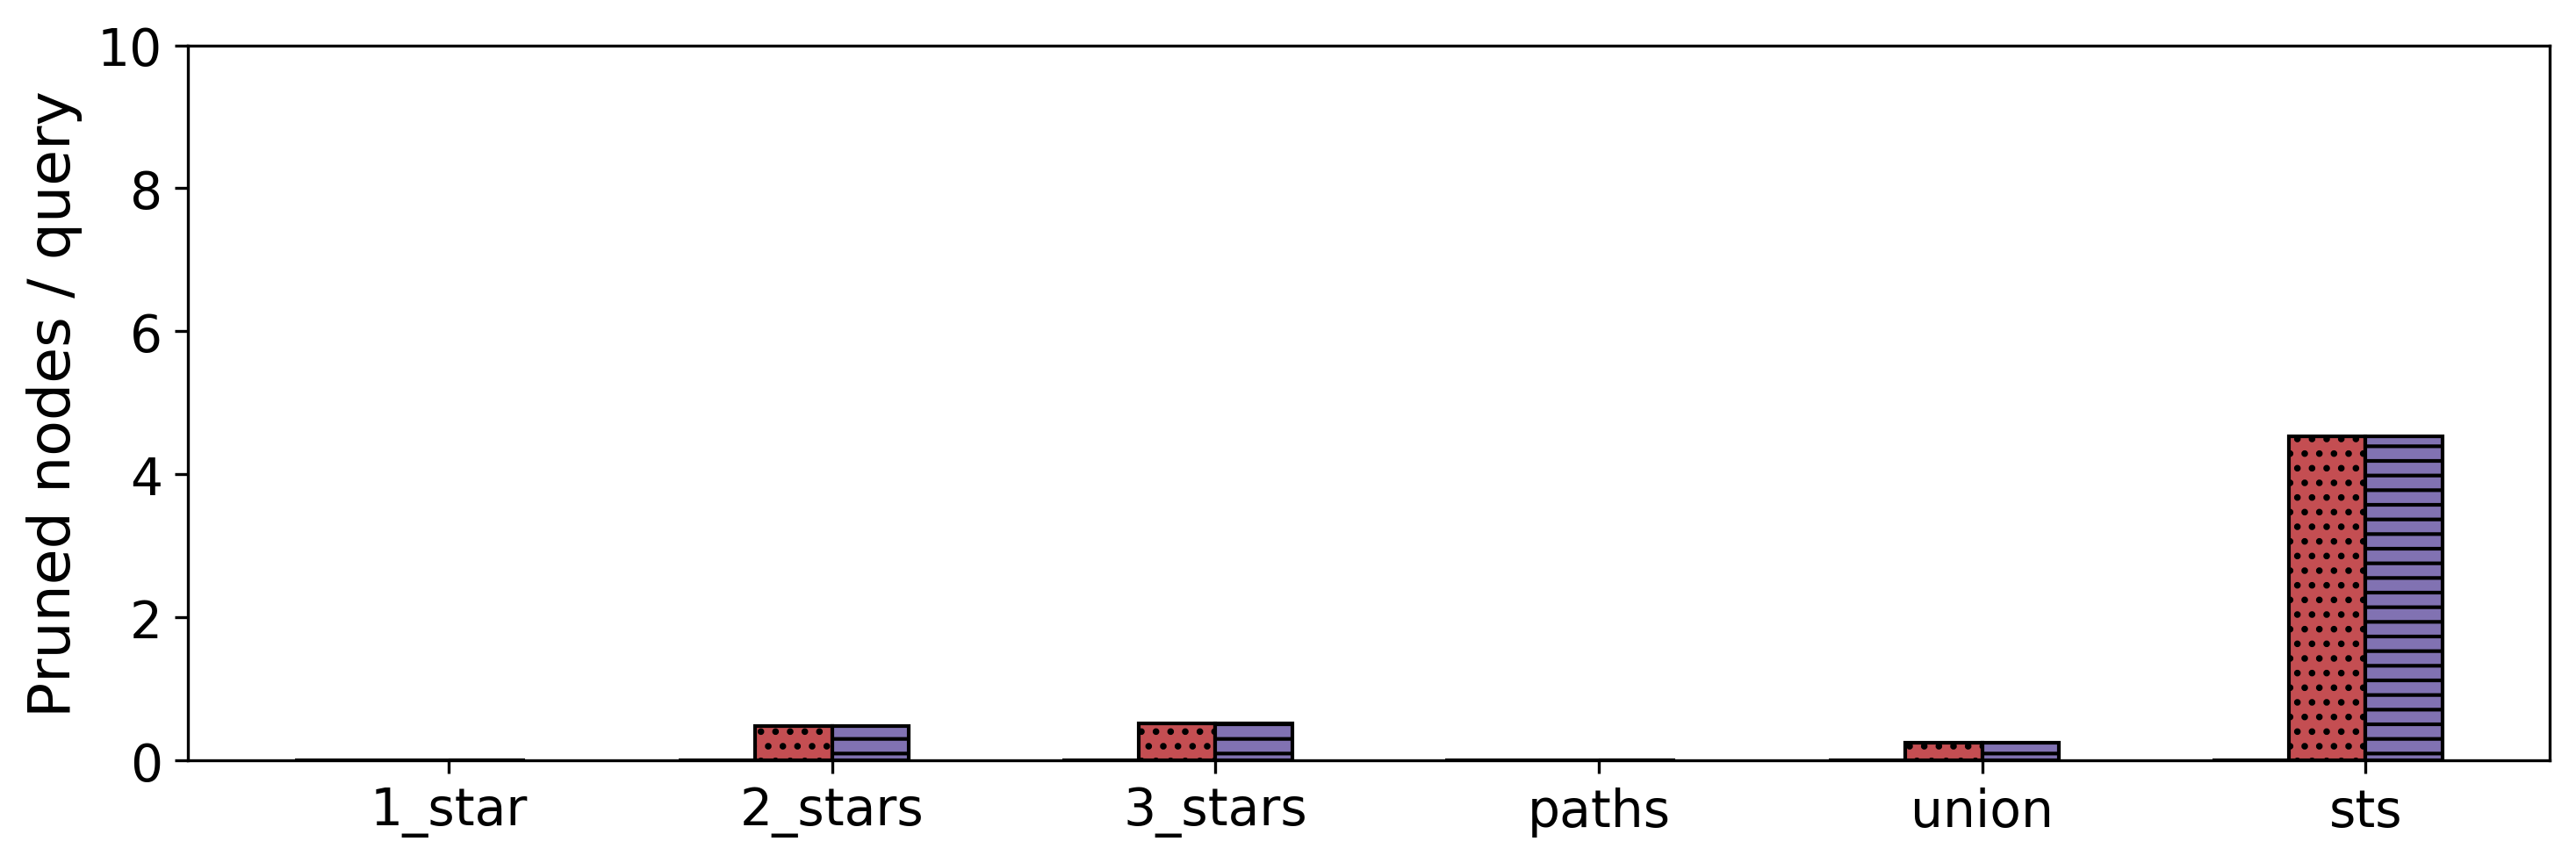}
  \caption{Number of pruned nodes per query over \texttt{watdiv1000M}}\label{subfig:appb:npn_1000M}
\end{subfigure}
\caption{Number of pruned fragments and nodes per query for the WatDiv datasets and star queries.}
\label{fig:appb:npf_npn}
\end{figure*}
