# Supplementary material for: The Lothbrok approach for SPARQL Query Optimization over Decentralized Knowledge Graphs
Source: arXiv:2208.14692 source file (2022-08-31)
Supplement: Supplementary file 2 [file appendix.tex]

In this appendix, we provide additional experimental results for the LargeRDFBench experiments.
Figure~\ref{fig:perf_s} shows QET, QRT, and QOT for the S query load,
Figure~\ref{fig:perf_l} for the L load, and
Figure~\ref{fig:perf_ch} for the CH load.

\begin{figure*}[tb!]
\centering
\includegraphics[width=.6\textwidth]{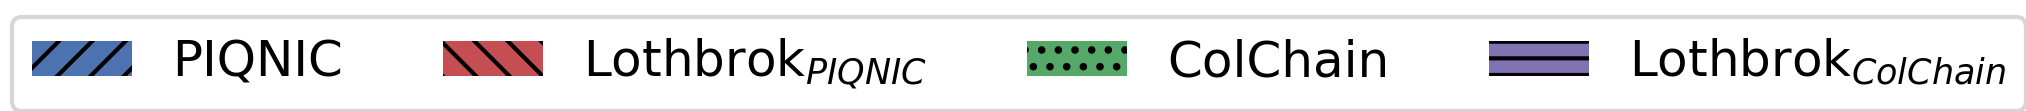}
%\vspace{-5ex}
\begin{subfigure}[b]{\textwidth}
  \includegraphics[width=\textwidth]{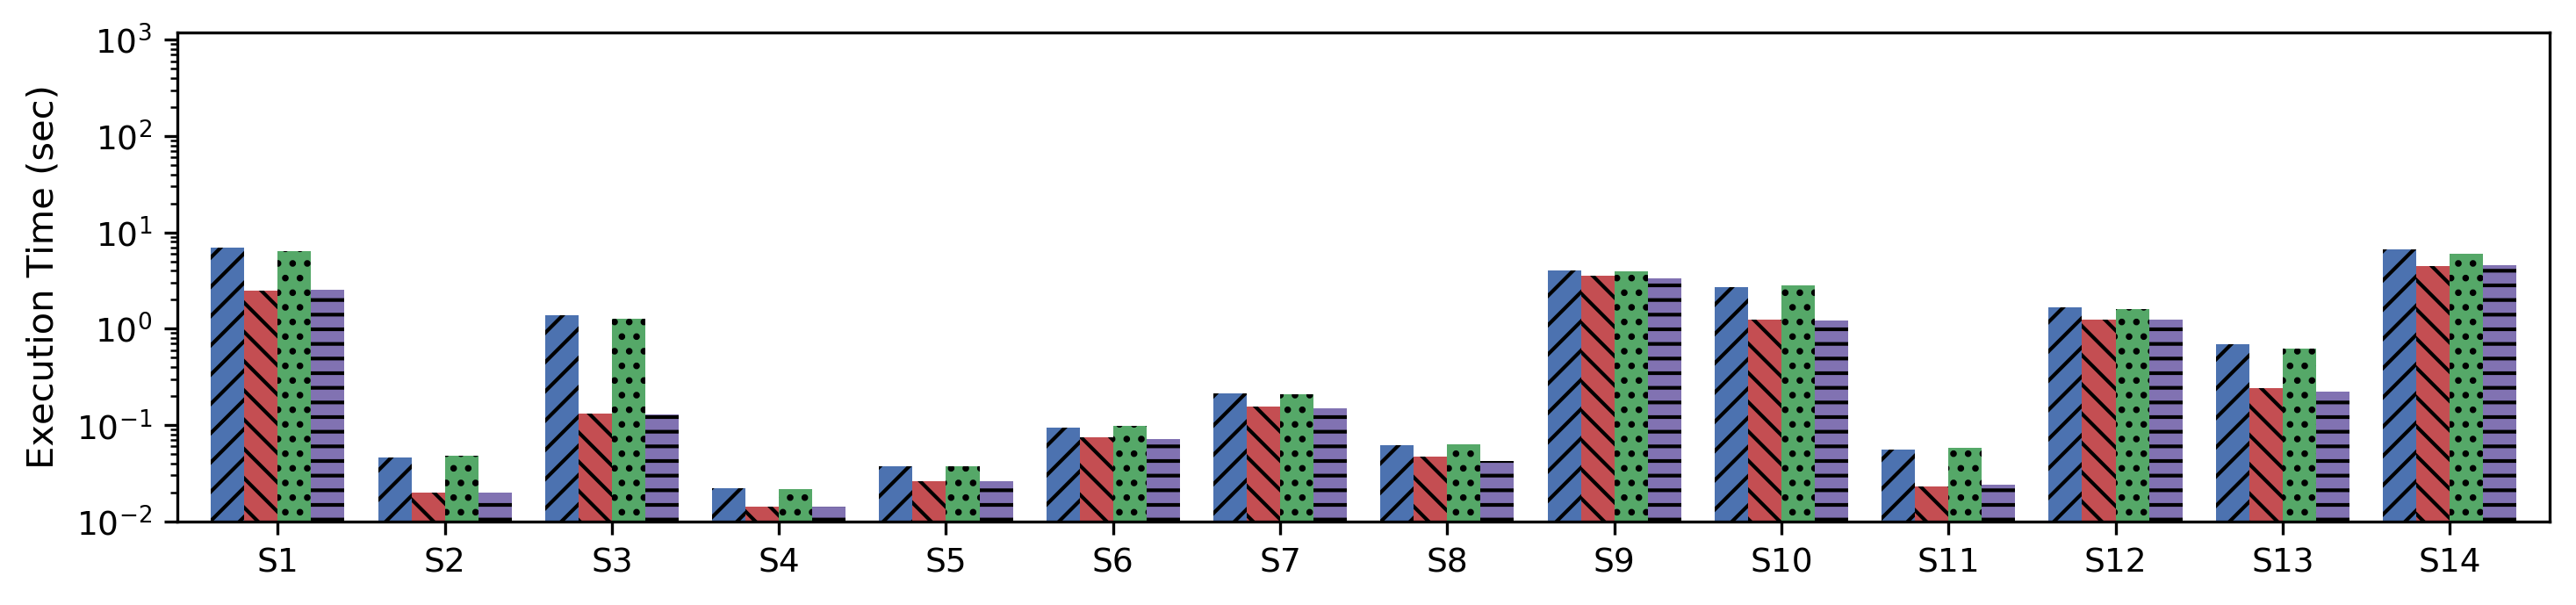}
  \caption{Execution time (QET)}\label{subfig:qet_s}
\end{subfigure}
\begin{subfigure}[b]{\textwidth}
  \includegraphics[width=\textwidth]{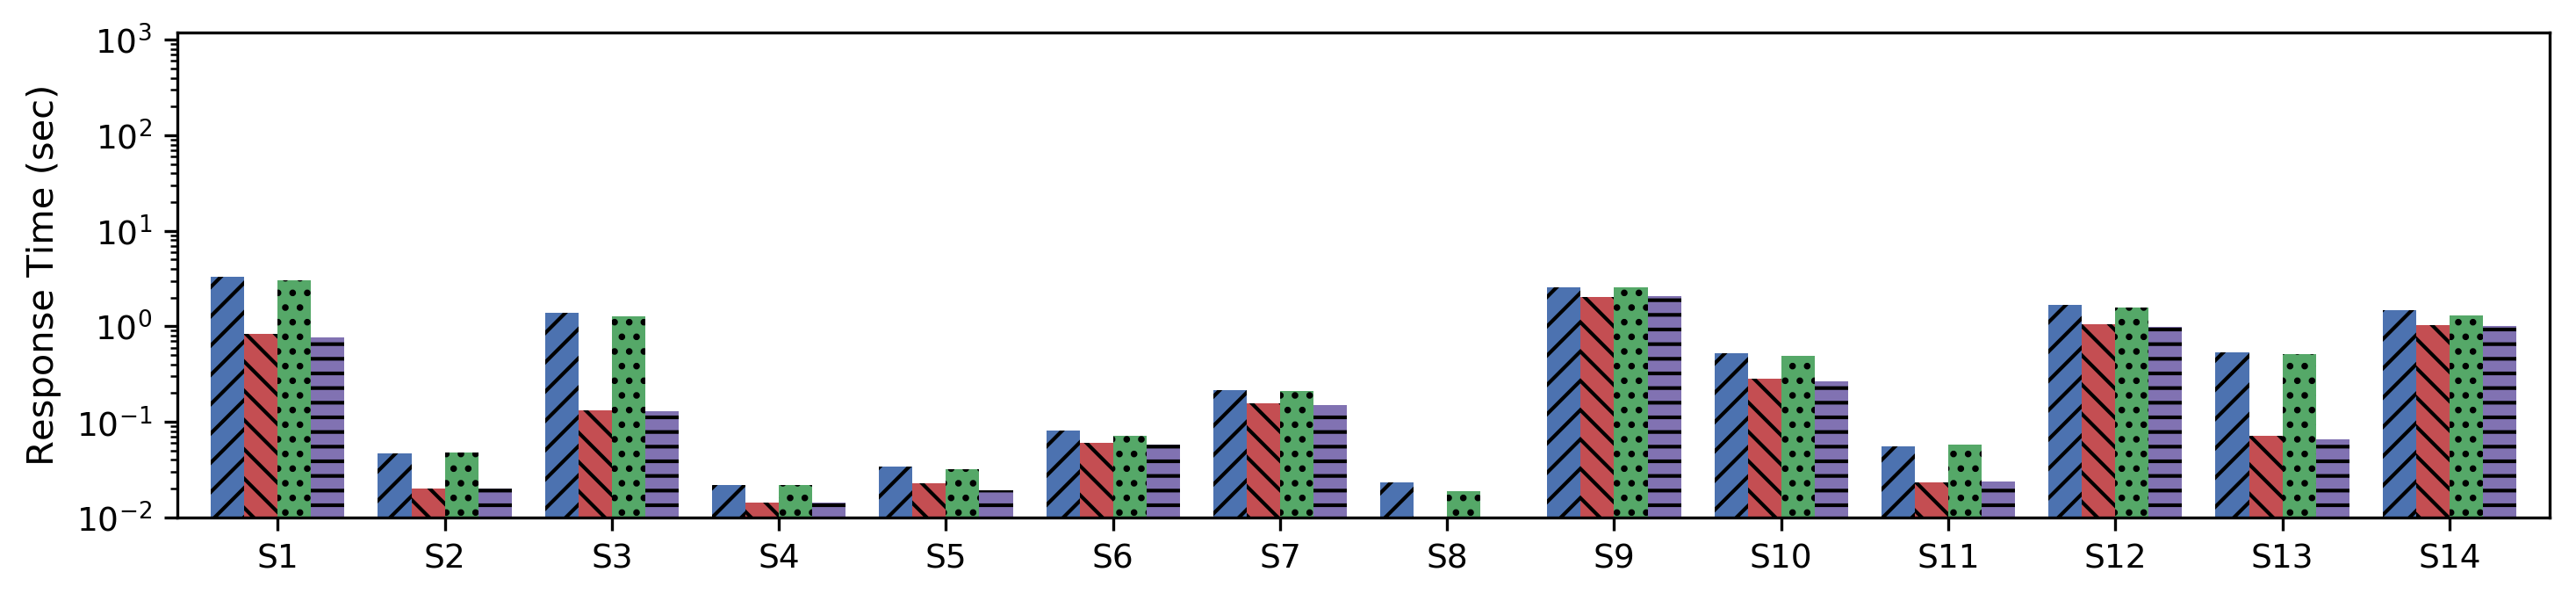}
  \caption{Response time (QRT)}\label{subfig:qrt_s}
\end{subfigure}
\begin{subfigure}[b]{\textwidth}
  \includegraphics[width=\textwidth]{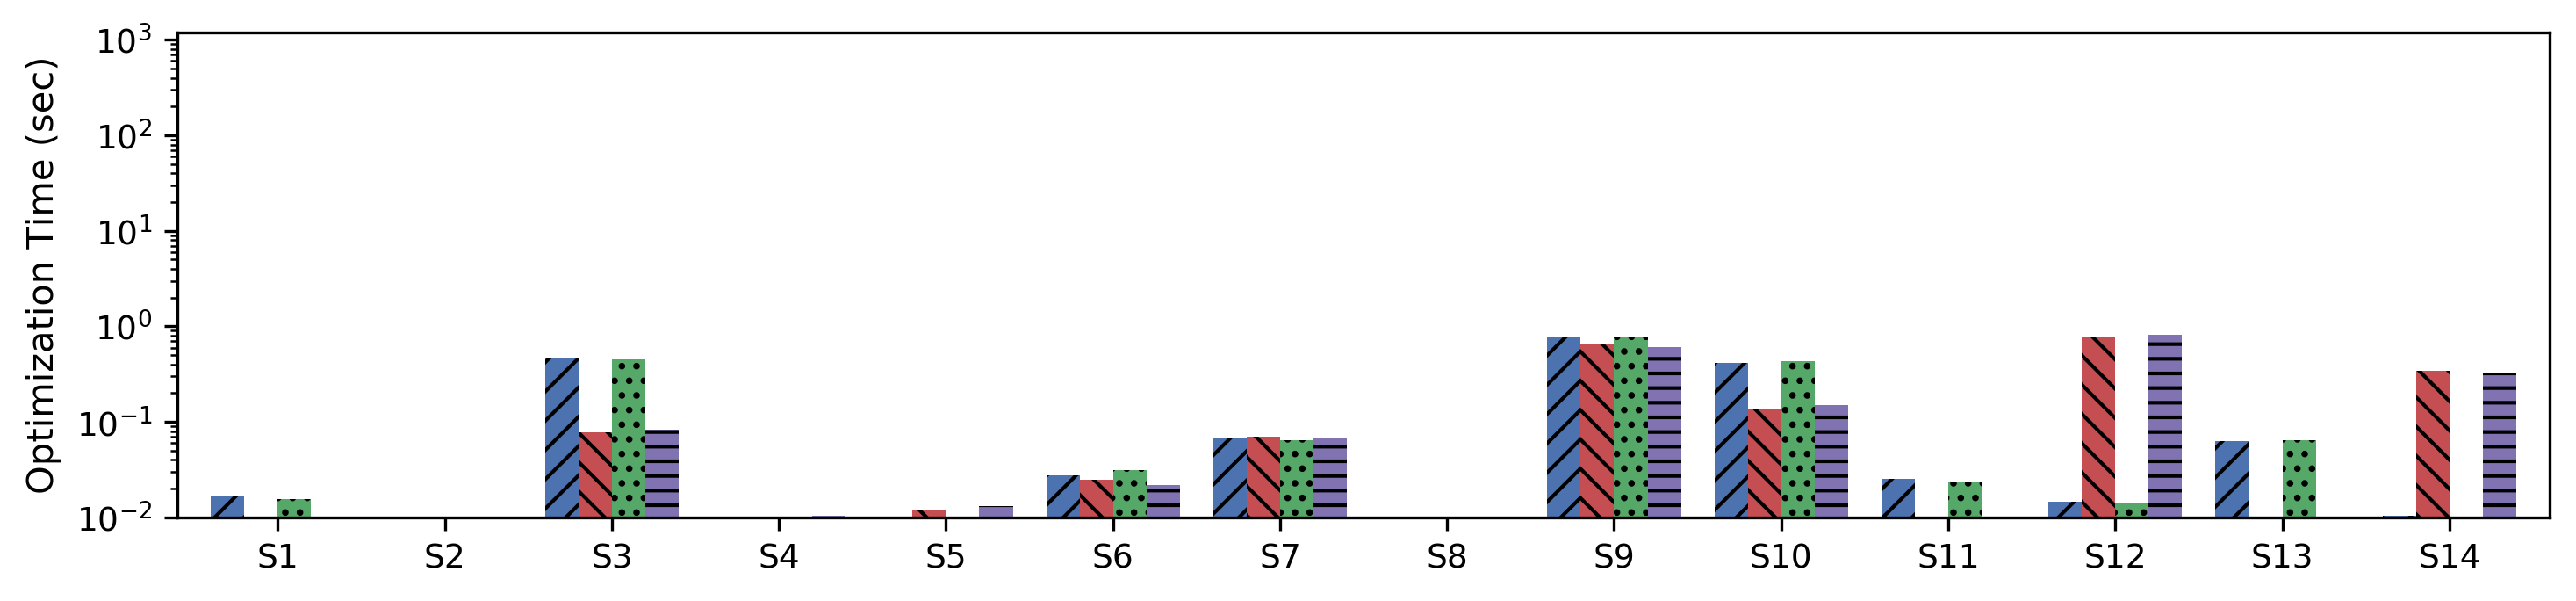}
  \caption{Optimization time (QOT)}\label{subfig:qot_s}
\end{subfigure}
\caption{Query execution time (a), response time (b), and optimization time (c) for the S query load over LargeRDFBench.}
\label{fig:perf_s}
\end{figure*}

\begin{figure*}[tb!]
\centering
\includegraphics[width=.6\textwidth]{figures/results/performance/legend1.png}
%\vspace{-5ex}
\begin{subfigure}[b]{\textwidth}
  \includegraphics[width=\textwidth]{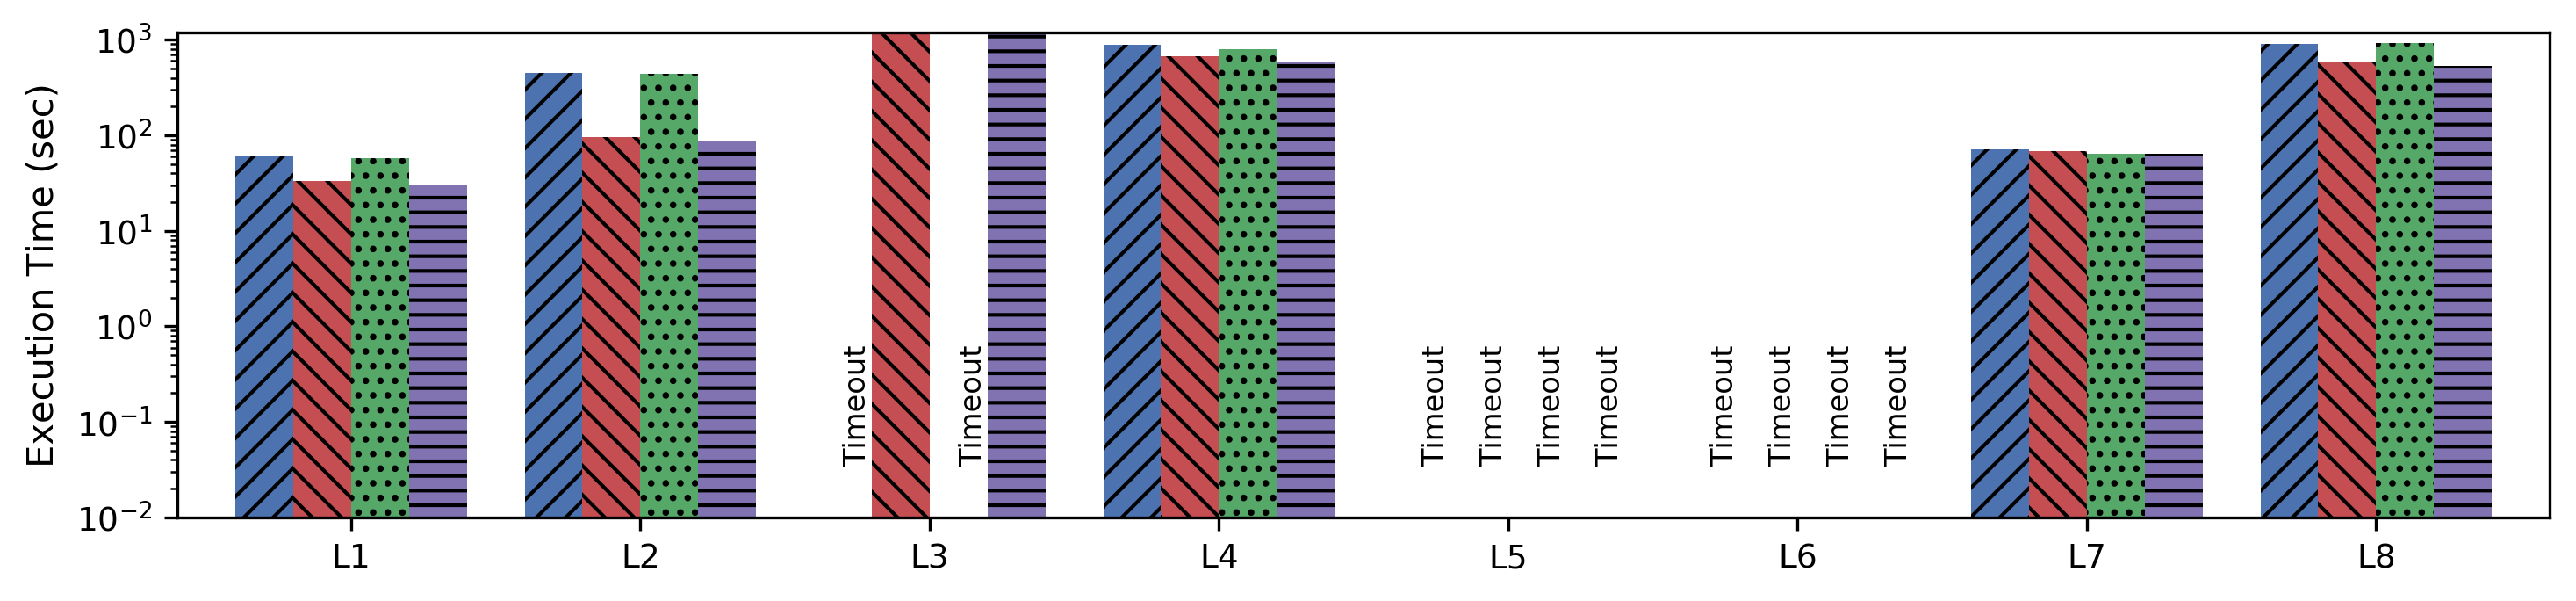}
  \caption{Execution time (QET)}\label{subfig:qet_l}
\end{subfigure}
\begin{subfigure}[b]{\textwidth}
  \includegraphics[width=\textwidth]{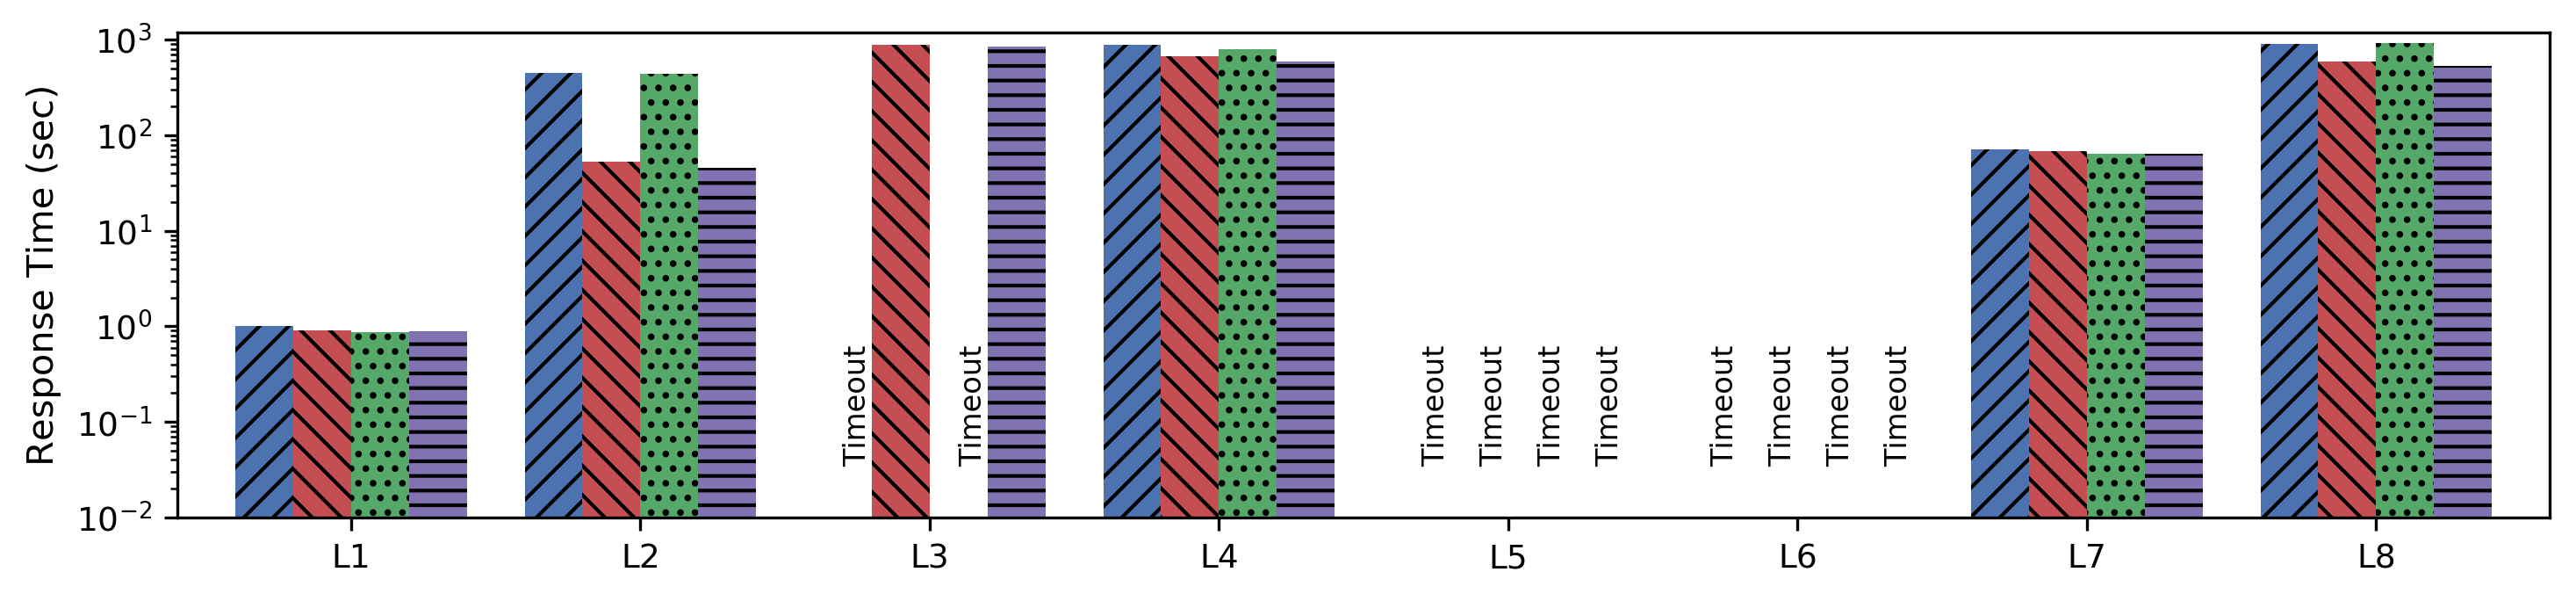}
  \caption{Response time (QRT)}\label{subfig:qrt_l}
\end{subfigure}
\begin{subfigure}[b]{\textwidth}
  \includegraphics[width=\textwidth]{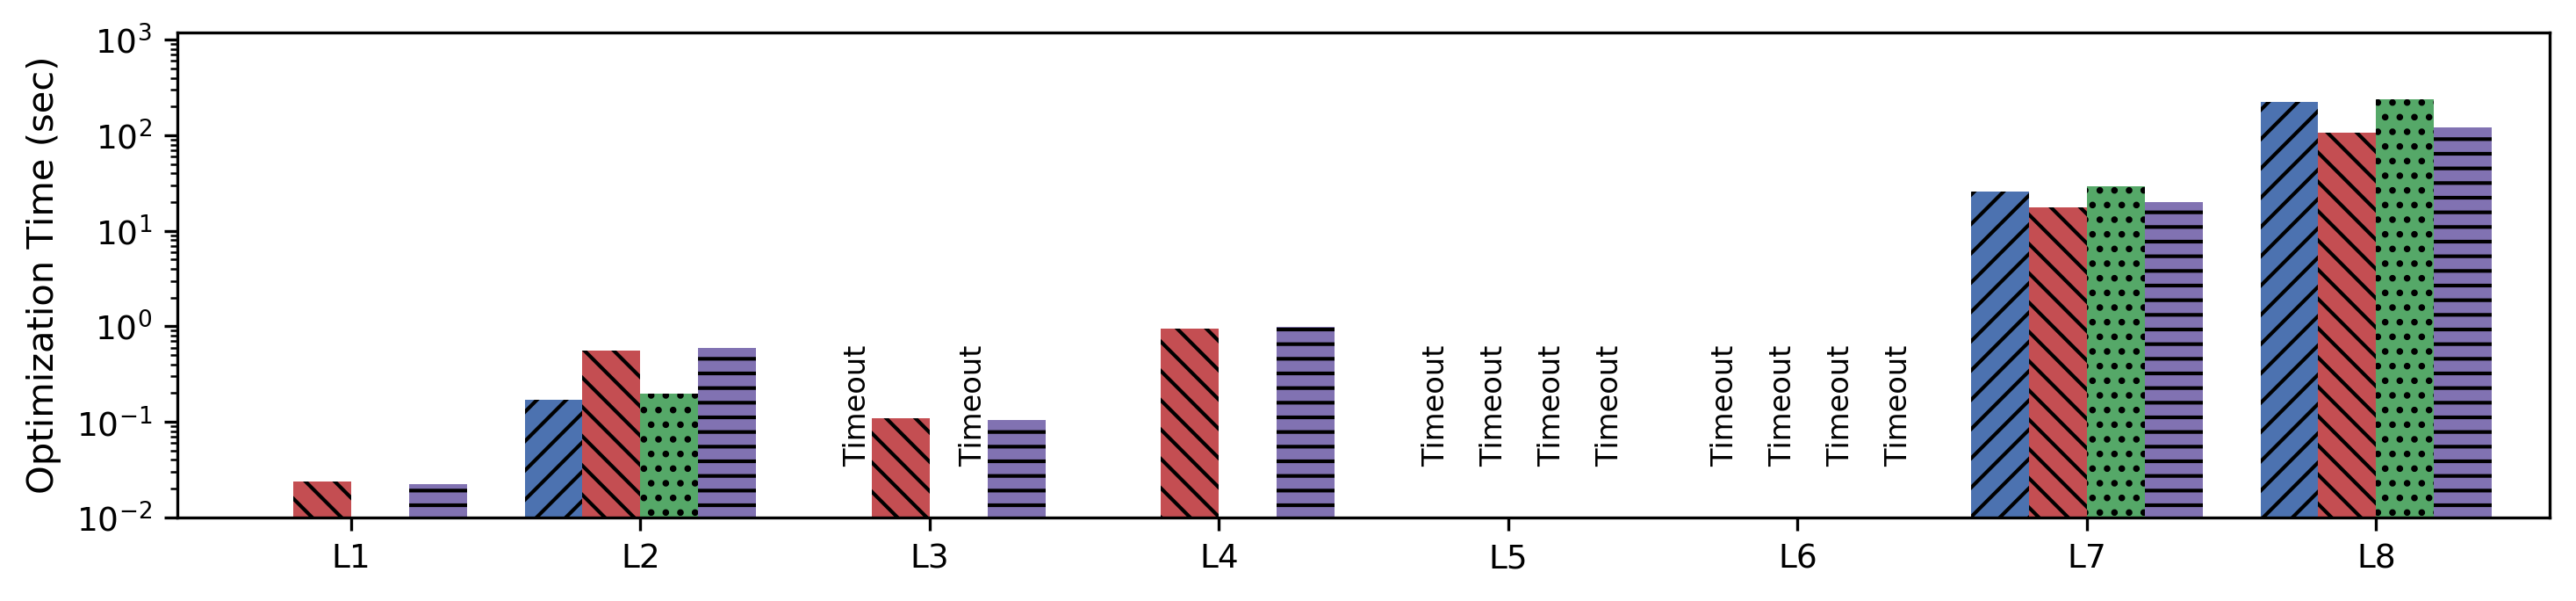}
  \caption{Optimization time (QOT)}\label{subfig:qot_l}
\end{subfigure}
\caption{Query execution time (a), response time (b), and optimization time (c) for the L query load over LargeRDFBench.}
\label{fig:perf_l}
\end{figure*}

\begin{figure*}[tb!]
\centering
\includegraphics[width=.6\textwidth]{figures/results/performance/legend1.png}
%\vspace{-5ex}
\begin{subfigure}[b]{\textwidth}
  \includegraphics[width=\textwidth]{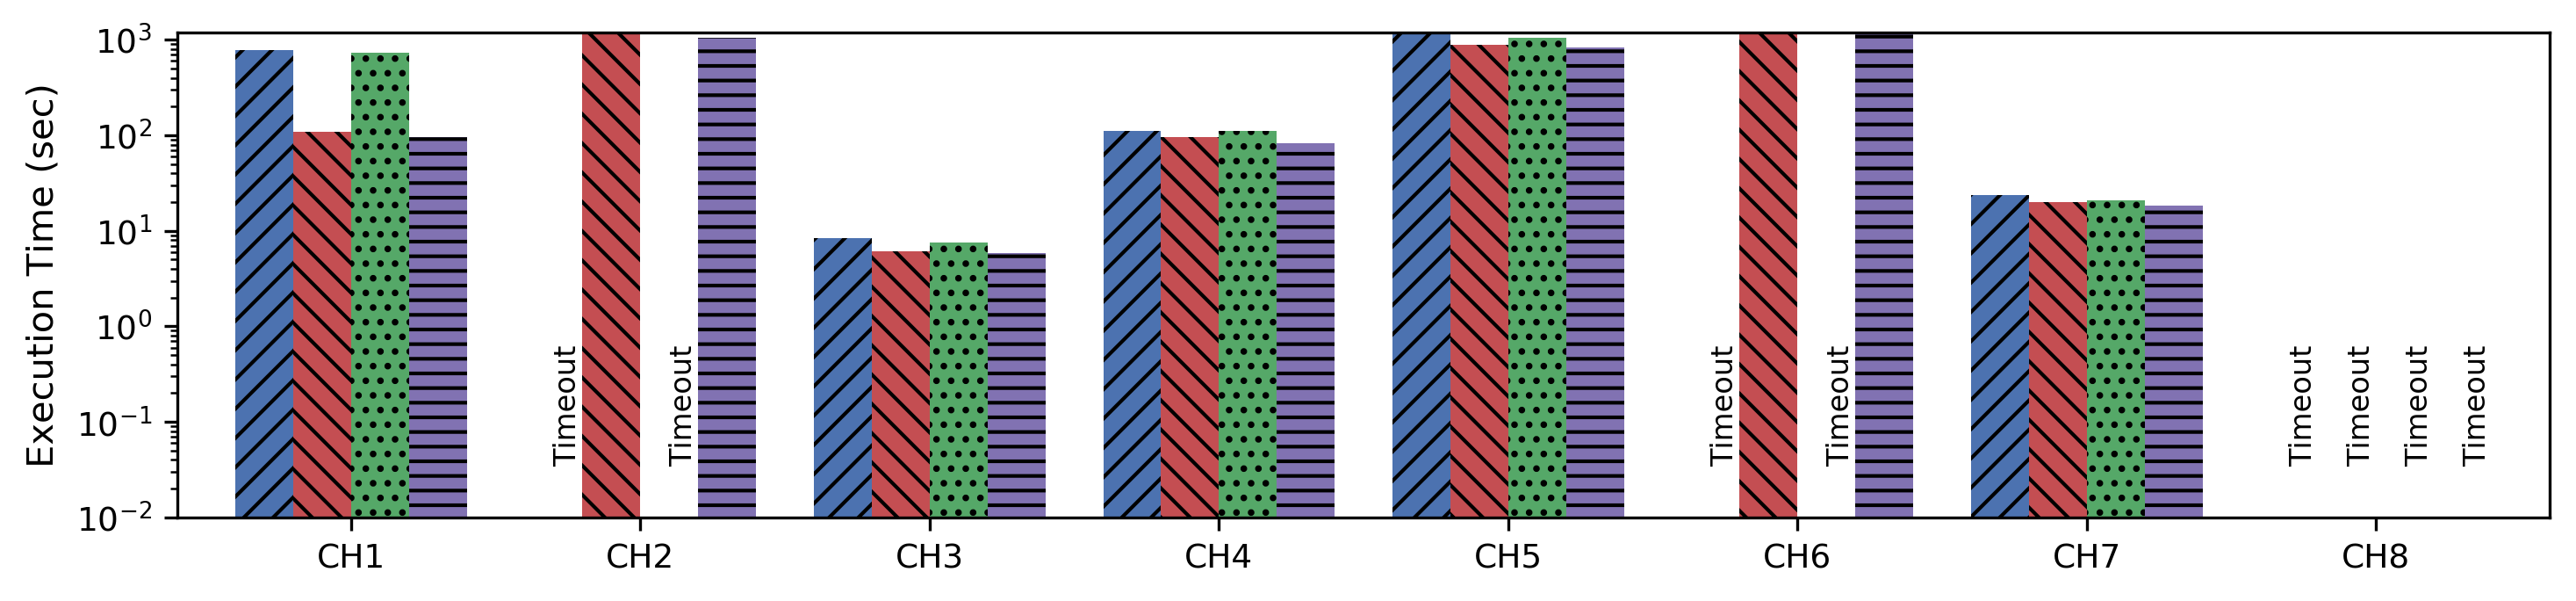}
  \caption{Execution time (QET)}\label{subfig:qet_ch}
\end{subfigure}
\begin{subfigure}[b]{\textwidth}
  \includegraphics[width=\textwidth]{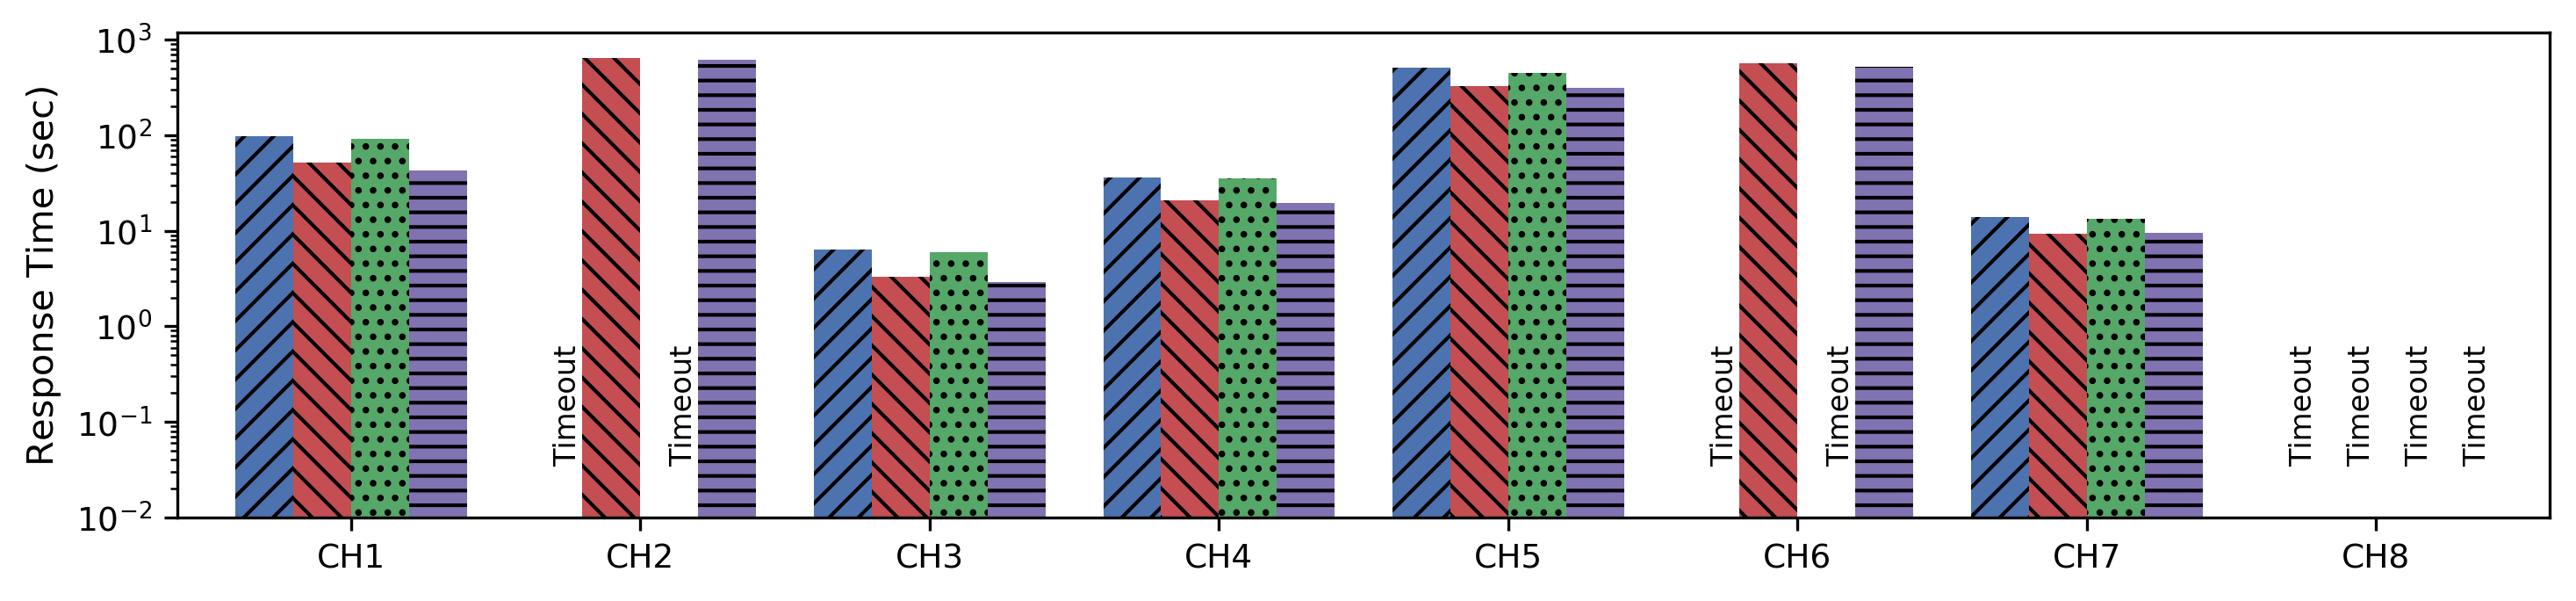}
  \caption{Response time (QRT)}\label{subfig:qrt_ch}
\end{subfigure}
\begin{subfigure}[b]{\textwidth}
  \includegraphics[width=\textwidth]{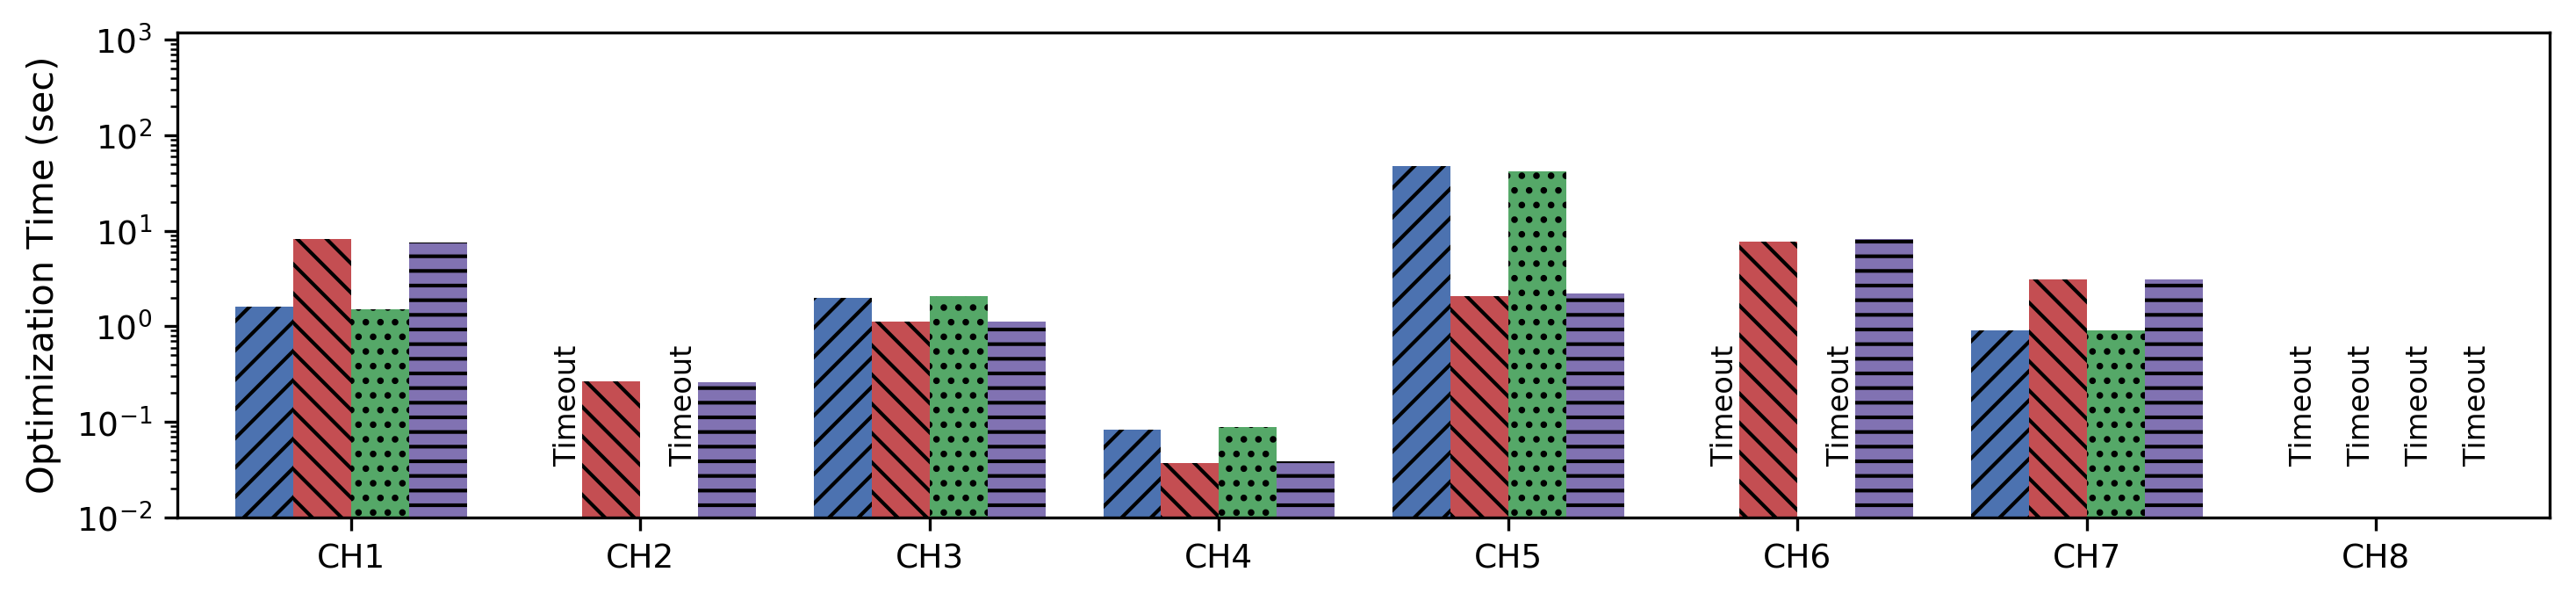}
  \caption{Optimization time (QOT)}\label{subfig:qot_ch}
\end{subfigure}
\caption{Query execution time (a), response time (b), and optimization time (c) for the CH query load over LargeRDFBench.}
\label{fig:perf_ch}
\end{figure*}
